# Supplementary material for: Sterile Neutrinos from Dark Matter: A $\nu$ Nightmare?
Source: arXiv:2211.05996 source file (2022-11-11)
Supplement: Supplementary file 1 [file mass_diag_approx.tex]

Here we diagonalize the neutrino mass matrix pertubatively. To do so, we assume that \(\norm{\hat{\bm{m}}_{D}} \ll \norm{\hat{\bm{m}}}\).
We introduce an ordering parameter \(\epsilon\) and let the mass matrix be
\begin{align}
	\hat{\bm{M}}             & = \mqty(
	\bm{0}_{3\times3}        & \epsilon\hat{\bm{m}}_{D} \\
	\epsilon\hat{\bm{m}}_{D} & \hat{\bm{m}}
	)
\end{align}
We then let
\begin{align}
	\OmegaVVb     & = \sum_{n}\bm{\cA}_{n}\epsilon^{n},       &
	\OmegaVNb     & = \sum_{n}\bm{\cB}_{n}\epsilon^{n},       &
	\OmegaNVb     & = \sum_{n}\bm{\cC}_{n}\epsilon^{n},       &
	\OmegaNNb     & = \sum_{n}\bm{\cD}_{n}\epsilon^{n}          \\
	\bm{m}_{\nu}  & = \sum_{n}\bm{m}_{\nu}^{(n)}\epsilon^{n}  &
	\bm{m}_{\rhn} & = \sum_{n}\bm{m}_{\rhn}^{(n)}\epsilon^{n}
\end{align}
We can then solve the diagonalization conditions order-by-order in \(\epsilon\). Our first equation is:
\begin{align}
	\bm{m}_{\nu}
	                   & =
	\OmegaVVb^{T}\hat{\bm{m}}_{D}\OmegaNVb+\OmegaNVb^{T}\hat{\bm{m}}^{T}_{D}\OmegaVVb+\OmegaNVb^{T}\hat{\bm{m}}\OmegaNVb \\
	\bm{m}^{(0)}_{\nu} & = \bm{\cC}_{0}^{T}\hat{\bm{m}}\bm{\cC}_{0}                                                      \\
	\bm{m}^{(1)}_{\nu} & =
	\bm{\cC}_{0}^{T}\hat{\bm{m}}_{D}\bm{\cA}_{0}
	+\bm{\cA}_{0}^{T}\hat{\bm{m}}_{D}\bm{\cC}_{0}
	+\bm{\cC}_{0}^{T}\hat{\bm{m}}\bm{\cC}_{1}
	+\bm{\cC}_{1}^{T}\hat{\bm{m}}\bm{\cC}_{0}
	%\\
	%\bm{m}^{(2)}_{\nu} & =
	%\bm{\cC}_{1}^{T}\hat{\bm{m}}_{D}\bm{\cA}_{0}
	%+ \bm{\cC}_{0}^{T}\hat{\bm{m}}_{D}\bm{\cA}_{1}
	%+\bm{\cA}_{1}^{T}\hat{\bm{m}}_{D}\bm{\cC}_{0}
	%+\bm{\cA}_{0}^{T}\hat{\bm{m}}_{D}\bm{\cC}_{1}
	%+\bm{\cC}_{2}^{T}\hat{\bm{m}}\bm{\cC}_{0}
	%+\bm{\cC}_{1}^{T}\hat{\bm{m}}\bm{\cC}_{1}
	%+\bm{\cC}_{0}^{T}\hat{\bm{m}}\bm{\cC}_{2}
\end{align}
Then next equation
\begin{align}
	\bm{m}_{\rhn}       & =
	\OmegaVNb^{T}\hat{\bm{m}}_{D}\OmegaNNb
	+\OmegaNNb^{T}\hat{\bm{m}}^{T}_{D}\OmegaVNb
	+\OmegaNNb^{T} \hat{\bm{m}}\OmegaNNb                             \\
	\bm{m}^{(0)}_{\rhn} & = \bm{\cD}_{0}^{T}\hat{\bm{m}}\bm{\cD}_{0} \\
	\bm{m}^{(1)}_{\rhn} & =
	\bm{\cD}_{0}^{T}\hat{\bm{m}}_{D}\bm{\cB}_{0}
	+\bm{\cB}_{0}^{T}\hat{\bm{m}}_{D}\bm{\cD}_{0}
	+\bm{\cD}_{0}^{T}\hat{\bm{m}}\bm{\cD}_{1}
	+\bm{\cD}_{1}^{T}\hat{\bm{m}}\bm{\cD}_{0}
	%\\
	%\bm{m}^{(2)}_{\rhn} & =
	%\bm{\cD}_{1}^{T}\hat{\bm{m}}_{D}\bm{\cB}_{0}
	%+ \bm{\cD}_{0}^{T}\hat{\bm{m}}_{D}\bm{\cB}_{1}
	%+\bm{\cB}_{1}^{T}\hat{\bm{m}}_{D}\bm{\cD}_{0}
	%+\bm{\cB}_{0}^{T}\hat{\bm{m}}_{D}\bm{\cD}_{1}
	%+\bm{\cD}_{2}^{T}\hat{\bm{m}}\bm{\cD}_{0}
	%+\bm{\cD}_{1}^{T}\hat{\bm{m}}\bm{\cD}_{1}
	%+\bm{\cD}_{0}^{T}\hat{\bm{m}}\bm{\cD}_{2}
\end{align}

\begin{align}
	\bm{0}_{3\times n} & =
	\OmegaNVb^{T}\hat{\bm{m}}^{T}_{D}\OmegaVNb+\OmegaVVb^{T}\hat{\bm{m}}_{D}\OmegaNNb+\OmegaNVb^{T}\hat{\bm{m}}\OmegaNNb \\
	0                  & = \bm{\cC}_{0}^{T}\hat{\bm{m}}\bm{\cD}_{0}                                                      \\
	0                  & =
	\bm{\cC}_{0}^{T}\hat{\bm{m}}_{D}\bm{\cB}_{0}
	+\bm{\cA}_{0}^{T}\hat{\bm{m}}_{D}\bm{\cD}_{0}
	+\bm{\cC}_{1}^{T}\hat{\bm{m}}\bm{\cD}_{0}
	+\bm{\cC}_{0}^{T}\hat{\bm{m}}\bm{\cD}_{1}
	%\\
	%\bm{m}^{(2)}_{\rhn} & =
	%\bm{\cD}_{1}^{T}\hat{\bm{m}}_{D}\bm{\cB}_{0}
	%+ \bm{\cD}_{0}^{T}\hat{\bm{m}}_{D}\bm{\cB}_{1}
	%+\bm{\cB}_{1}^{T}\hat{\bm{m}}_{D}\bm{\cD}_{0}
	%+\bm{\cB}_{0}^{T}\hat{\bm{m}}_{D}\bm{\cD}_{1}
	%+\bm{\cD}_{2}^{T}\hat{\bm{m}}\bm{\cD}_{0}
	%+\bm{\cD}_{1}^{T}\hat{\bm{m}}\bm{\cD}_{1}
	%+\bm{\cD}_{0}^{T}\hat{\bm{m}}\bm{\cD}_{2}
\end{align}

\begin{align}
	\bm{1} & = \OmegaVVb^{\dagger}\OmegaVVb + \OmegaNVb^{\dagger}\OmegaNVb             \\
	1      & = \bm{\cA}_{0}^{\dagger}\bm{\cA}_{0} + \bm{\cC}_{0}^{\dagger}\bm{\cC}_{0} \\
	0      & =
	\bm{\cA}_{1}^{\dagger}\bm{\cA}_{0} +
	\bm{\cA}_{0}^{\dagger}\bm{\cA}_{1} +
	\bm{\cC}_{1}^{\dagger}\bm{\cC}_{0} +
	\bm{\cC}_{0}^{\dagger}\bm{\cC}_{1}
	%\\
	%\bm{m}^{(2)}_{\rhn} & =
	%\bm{\cD}_{1}^{T}\hat{\bm{m}}_{D}\bm{\cB}_{0}
	%+ \bm{\cD}_{0}^{T}\hat{\bm{m}}_{D}\bm{\cB}_{1}
	%+\bm{\cB}_{1}^{T}\hat{\bm{m}}_{D}\bm{\cD}_{0}
	%+\bm{\cB}_{0}^{T}\hat{\bm{m}}_{D}\bm{\cD}_{1}
	%+\bm{\cD}_{2}^{T}\hat{\bm{m}}\bm{\cD}_{0}
	%+\bm{\cD}_{1}^{T}\hat{\bm{m}}\bm{\cD}_{1}
	%+\bm{\cD}_{0}^{T}\hat{\bm{m}}\bm{\cD}_{2}
\end{align}

\begin{align}
	\bm{1} & = \OmegaNNb^{\dagger}\OmegaNNb + \OmegaVNb^{\dagger}\OmegaVNb             \\
	1      & = \bm{\cD}_{0}^{\dagger}\bm{\cD}_{0} + \bm{\cB}_{0}^{\dagger}\bm{\cB}_{0} \\
	0      & =
	\bm{\cD}_{1}^{\dagger}\bm{\cD}_{0} +
	\bm{\cD}_{0}^{\dagger}\bm{\cD}_{1} +
	\bm{\cB}_{1}^{\dagger}\bm{\cB}_{0} +
	\bm{\cB}_{0}^{\dagger}\bm{\cB}_{1}
	%\\
	%\bm{m}^{(2)}_{\rhn} & =
	%\bm{\cD}_{1}^{T}\hat{\bm{m}}_{D}\bm{\cB}_{0}
	%+ \bm{\cD}_{0}^{T}\hat{\bm{m}}_{D}\bm{\cB}_{1}
	%+\bm{\cB}_{1}^{T}\hat{\bm{m}}_{D}\bm{\cD}_{0}
	%+\bm{\cB}_{0}^{T}\hat{\bm{m}}_{D}\bm{\cD}_{1}
	%+\bm{\cD}_{2}^{T}\hat{\bm{m}}\bm{\cD}_{0}
	%+\bm{\cD}_{1}^{T}\hat{\bm{m}}\bm{\cD}_{1}
	%+\bm{\cD}_{0}^{T}\hat{\bm{m}}\bm{\cD}_{2}
\end{align}

\begin{align}
	\bm{0} & = \OmegaVNb^{\dagger}\OmegaVVb + \OmegaNNb^{\dagger}\OmegaNVb             \\
	0      & = \bm{\cB}_{0}^{\dagger}\bm{\cA}_{0} + \bm{\cD}_{0}^{\dagger}\bm{\cC}_{0} \\
	0      & =
	\bm{\cB}_{1}^{\dagger}\bm{\cA}_{0} +
	\bm{\cB}_{0}^{\dagger}\bm{\cA}_{1} +
	\bm{\cD}_{1}^{\dagger}\bm{\cC}_{0} +
	\bm{\cD}_{0}^{\dagger}\bm{\cC}_{1}
	%\\
	%\bm{m}^{(2)}_{\rhn} & =
	%\bm{\cD}_{1}^{T}\hat{\bm{m}}_{D}\bm{\cB}_{0}
	%+ \bm{\cD}_{0}^{T}\hat{\bm{m}}_{D}\bm{\cB}_{1}
	%+\bm{\cB}_{1}^{T}\hat{\bm{m}}_{D}\bm{\cD}_{0}
	%+\bm{\cB}_{0}^{T}\hat{\bm{m}}_{D}\bm{\cD}_{1}
	%+\bm{\cD}_{2}^{T}\hat{\bm{m}}\bm{\cD}_{0}
	%+\bm{\cD}_{1}^{T}\hat{\bm{m}}\bm{\cD}_{1}
	%+\bm{\cD}_{0}^{T}\hat{\bm{m}}\bm{\cD}_{2}
\end{align}

To order \(\epsilon^{0}\), we have:
\begin{align}
	\bm{m}^{(0)}_{\nu}  & = \bm{\cC}_{0}^{T}\hat{\bm{m}}\bm{\cC}_{0}                                \\
	\bm{m}^{(0)}_{\rhn} & = \bm{\cD}_{0}^{T}\hat{\bm{m}}\bm{\cD}_{0}                                \\
	0                   & = \bm{\cC}_{0}^{T}\hat{\bm{m}}\bm{\cD}_{0}                                \\
	1                   & = \bm{\cA}_{0}^{\dagger}\bm{\cA}_{0} + \bm{\cC}_{0}^{\dagger}\bm{\cC}_{0} \\
	1                   & = \bm{\cD}_{0}^{\dagger}\bm{\cD}_{0} + \bm{\cB}_{0}^{\dagger}\bm{\cB}_{0} \\
	0                   & = \bm{\cB}_{0}^{\dagger}\bm{\cA}_{0} + \bm{\cD}_{0}^{\dagger}\bm{\cC}_{0}
\end{align}
Assuming \(\hat{\bm{m}}\) is diagonal, we find that
\begin{align}
	\bm{\cA}            & = \bm{1}       &
	\bm{\cB}            & = \bm{0}       &
	\bm{\cC}            & = \bm{0}       &
	\bm{\cD}            & = \bm{1}         \\
	\bm{m}^{(0)}_{\nu}  & = \bm{0}       &
	\bm{m}^{(0)}_{\rhn} & = \hat{\bm{m}}
\end{align}
To order \(\epsilon^{1}\), we have:
\begin{align}
	\bm{m}^{(1)}_{\nu}  & = \bm{0} \\
	%--------------
	\bm{m}^{(1)}_{\rhn} & =
	\hat{\bm{m}}\bm{\cD}_{1}
	+\bm{\cD}_{1}^{T}\hat{\bm{m}}  \\
	%--------------
	0                   & =
	\hat{\bm{m}}_{D}
	+\bm{\cC}_{1}^{T}\hat{\bm{m}}  \\
	%--------------
	0                   & =
	\bm{\cA}_{1}^{\dagger} +
	\bm{\cA}_{1}                   \\
	%--------------
	0                   & =
	\bm{\cD}_{1}^{\dagger} +
	\bm{\cD}_{1}                   \\
	%--------------
	0                   & =
	\bm{\cB}_{1}^{\dagger} +
	\bm{\cC}_{1}
\end{align}

Thus,
\begin{align}
	\bm{m}^{(1)}_{\nu}  & = \bm{0} \\
	%--------------
	\bm{m}^{(1)}_{\rhn} & =
	\hat{\bm{m}}\bm{\cD}_{1}
	+\bm{\cD}_{1}^{T}\hat{\bm{m}}  \\
	%--------------
	\bm{\cC}_{1}^{T}    & =
	-\hat{\bm{m}}_{D}\hat{\bm{m}}^{-1}
	\\
	%--------------
	0                   & =
	\bm{\cD}_{1}^{\dagger} +
	\bm{\cD}_{1}                   \\
	%--------------
	\bm{\cB}_{1}^{*}    & =
	\hat{\bm{m}}_{D}\hat{\bm{m}}^{-1}
\end{align}

To order \(\epsilon^{2}\), we have:
\begin{align}
	\bm{m}^{(2)}_{\nu}  & =
	-\hat{\bm{m}}_{D}\hat{\bm{m}}^{-1}
	\hat{\bm{m}}^{T}_{D}    \\
	\bm{m}^{(2)}_{\rhn} & =
	+ \hat{\bm{m}}_{D}\bm{\cB}_{1}
	+\bm{\cB}_{1}^{T}\hat{\bm{m}}_{D}
	+\bm{\cD}_{2}^{T}\hat{\bm{m}}
	+\bm{\cD}_{1}^{T}\hat{\bm{m}}\bm{\cD}_{1}
	+\hat{\bm{m}}\bm{\cD}_{2}
\end{align}
