# Supplementary material for: Sterile Neutrinos from Dark Matter: A $\nu$ Nightmare?
Source: arXiv:2211.05996 source file (2022-11-11)
Supplement: Supplementary file 2 [file appendix_chiral_lagrangian.tex]

\section{Matching Onto Chiral Lagrangian}

In this appendix, we show how to match the RH neutrino Lagragian onto the chiral
Lagragian to obtain interactions containings the RH neutrino and mesons.

\subsection{Leading Order Chiral Lagrangian}

Recall that the leading-order chiral Lagrangian is given by:
\begin{align}
    \cL_{\ChiPT} & = \frac{f_{\pi}^{2}}{4}\Tr[
        \qty(D_{\mu}\bm{\Sigma})^{\dagger}
        \qty(D^{\mu}\bm{\Sigma})
    ]
    + \frac{f_{\pi}^{2}}{4}\Tr[\bm{\chi}\bm{\Sigma}^{\dagger} + \mathrm{c.c.}]
\end{align}
where \(f_{\pi}\) is the pion decay constant, \(\bm{\Sigma}\) is the Goldstone
matrix \(\exp(i\frac{i}{f_{\pi}}\phi_{a}\bm{\lambda}_{a})\),
\(D_{\mu}\) is the chiral covariant derivative, and
\(\bm{\chi} = 2B_{0}\bm{M}_{q}\). The \(\phi_{a}\) fields are such that
\begin{align}
    \phi_{a}\bm{\lambda}_{a} =
    \mqty(
    \pi^{0} + \eta/\sqrt{3} & \sqrt{2}\pi^{+}         & \sqrt{2}k^{+}           \\
    \sqrt{2}\pi^{-}         & -\pi^{0} +\eta/\sqrt{3} & \sqrt{2}k^{0}           \\
    \sqrt{2}k^{-}           & \sqrt{2}\bar{k}^{0}     & -\sqrt{\frac{2}{3}}\eta \\
    )
\end{align}
with \(\bm{\lambda}_{a}\) being the Gell-Mann matrices. The chiral covariant
derivative is given by:
\begin{align}
    D_{\mu}\bm{\Sigma} = \partial_{\mu}\bm{\Sigma} - i\bm{R}_{\mu}\bm{\Sigma} + i\bm{\Sigma}\bm{L}_{\mu}
\end{align}
with \(\bm{R}_{\mu}\) and \(\bm{L}_{\mu}\) the right and left handed quark currents.
The Goldstone matrix can be expanded in terms of the \(\phi\) fields and the Gell-Mann
matrices. If we write \(\bm{\Sigma} = \Sigma_{0}\bm{I} + \Sigma_{a}\bm{\lambda}_{a}\),
then:
\begin{align}
    \Sigma_{0}
     & =
    1
    + \frac{2}{3}S_{2}\expval{\phi^2}
    + \frac{2}{3}S_{3}\expval{\phi^3 d}
    + \frac{2}{3}S_{4}\expval{\phi^2}^{2}
    + \cdots \\
    \Sigma_{a}
     & =
    S_{1}\phi_{k}
    + S_{2}\expval{\phi^{2}d}_{k}
    + S_{3}\expval{\phi^{2}} \phi_{k}
    + S_{4}\qty(\frac{2}{3}\expval{\phi^{3}d}\phi_{k} + \expval{\phi}^{2}\expval{\phi^{2}d}_{k})
    + \cdots
\end{align}
where \(S_{n} = \frac{1}{n!}\qty(\frac{i}{f_{\pi}})^{n}\) and
\begin{align}
    \expval{\phi^{2}}
     & \equiv
    \phi_{a}\phi_{a},
     &
    \expval{\phi^{2}d}_{k}
     & \equiv
    \phi_{a}\phi_{b}d^{abk},
     &
    \expval{\phi^{3}d}
     & \equiv
    \phi_{a}\phi_{b}\phi_{c}d^{abc}
\end{align}
with \(d^{abc} = \frac{1}{4}\Tr[\bm{\lambda}_{a}\acomm{\bm{\lambda}_{b}}{\bm{\lambda}_{c}}]\).
The chiral kinetic term can be written as
\begin{align}
    \Tr[
        \qty(D_{\mu}\bm{\Sigma})^{\dagger}
        \qty(D^{\mu}\bm{\Sigma})
    ] = T_{2} + T_{3} + T_{4}
\end{align}
where
\begin{align}
    T_{2} & = \Tr[
        \qty(\partial_{\mu}\bm{\Sigma})^{\dagger}
        \qty(\partial_{\mu}\bm{\Sigma})
        + \bm{R}^{\dagger}_{\mu}\bm{R}_{\mu}
        + \bm{L}^{\dagger}_{\mu}\bm{L}_{\mu}
    ]               \\
    T_{3} & = i\Tr[
        \qty(\partial_{\mu}\bm{\Sigma})^{\dagger}
        \qty(
        \bm{\Sigma}\bm{L}_{\mu} -
        \bm{R}_{\mu}\bm{\Sigma}
        ) + \mathrm{c.c.}
    ]               \\
    T_{4} & = -\Tr[
        \bm{\Sigma}
        \bm{L}_{\mu}
        \bm{\Sigma}^{\dagger}
        \bm{R}^{\dagger}_{\mu}
    ]-\Tr[
        \bm{R}_{\mu}
        \bm{\Sigma}
        \bm{L}^{\dagger}_{\mu}
        \bm{\Sigma}^{\dagger}
    ]
\end{align}
If we define
\(\bm{L}_{\mu} = L_{\mu}^{0}\bm{I} + L^{a}_{\mu}\bm{\lambda}_{a}\) and
\(\bm{R}_{\mu} = R_{\mu}^{0}\bm{I} + R^{a}_{\mu}\bm{\lambda}_{a}\), then
\(T_{2}\) is
\begin{align}
    T_{2} & =
    3\qty(\qty|\partial_{\mu}\Sigma_{0}|^{2} + \qty|R^{0}_{\mu}|^{2} + \qty|L^{0}_{\mu}|^{2})
    +
    2\qty(\qty|\partial_{\mu}\Sigma_{a}|^{2} + \qty|R^{a}_{\mu}|^{2}+ \qty|L^{a}_{\mu}|^{2})
\end{align}
The second term is given by:
\begin{align}
    T_{3}
     & =
    3i\qty(L^{0}_{\mu}-R^{0}_{\mu})\Sigma_{0}\qty(\partial^{\mu}\Sigma_{0})^{\dagger} \\
     & \quad
    + 2i\qty[
        \qty(L^{a}_{\mu}-R^{a}_{\mu})
        \qty[
            \Sigma^{a}\qty(\partial^{\mu}\Sigma^{0})^{\dagger} +
            \Sigma^{0}\qty(\partial^{\mu}\Sigma^{a})^{\dagger}
        ] +
        \qty(L^{0}_{\mu}-R^{0}_{\mu})\Sigma^{a}\qty(\partial^{\mu}\Sigma^{a})^{\dagger}
    ]\notag                                                                           \\
     & \quad
    +2i\qty[
    \qty(L^{a}_{\mu}-R^{a}_{\mu})\Sigma^{b}\qty(\partial^{\mu}\Sigma^{c})^{\dagger}d_{abc} +
    i\qty(L^{a}_{\mu}+R^{a}_{\mu})\Sigma^{b}\qty(\partial^{\mu}\Sigma^{c})^{\dagger}f_{abc}
    ]\notag                                                                           \\
     & \quad
    + \mathrm{c.c.}\notag
\end{align}
The last term is given by
\begin{align}
    T_{4}
     & =
    \qty(3\qty|\Sigma_0|^{\dagger} + 2\Sigma^{\dagger}_{a}\Sigma_{a})R^{\dagger}_{0}L_{0}
    + 2\qty|\Sigma_{0}|^{2}R^{a}_{\mu}L_{a}               \\
     & \quad +
    2\qty(
    \Sigma_{0}\Sigma^{\dagger}_{a}
    +\Sigma_{a}\Sigma^{\dagger}_{0}
    )
    \qty(R^{a}_{\mu}L_{0} + R^{0}_{\mu}L^{a}_{\mu})\notag \\
     & \quad +
    2\qty[
    \Sigma^{\dagger}_{a}\qty(R^{b}_{\mu})^{\dagger}\Sigma_{c}L^{0}_{\mu} +
    \Sigma^{\dagger}_{a}\qty(R^{0}_{\mu})^{\dagger}\Sigma_{b}L^{c}_{\mu} +
    \Sigma^{\dagger}_{a}\qty(R^{b}_{\mu})^{\dagger}\Sigma_{0}L^{c}_{\mu} +
    \Sigma^{\dagger}_{0}\qty(R^{a}_{\mu})^{\dagger}\Sigma_{b}L^{c}_{\mu}
    ]\qty(d^{abc} + if^{abc})
    \notag                                                \\
     & \quad
    + \frac{4}{3}\Sigma^{\dagger}_{a}\qty(R^{a}_{\mu})^{\dagger}\Sigma_{b}L^{b}_{\mu}
    + 2\Sigma^{\dagger}_{a}\qty(R^{b}_{\mu})^{\dagger}\Sigma_{c}L^{d}_{\mu}
    \qty(d^{abe} +i f^{abe} )
    \qty(d^{cde} +i f^{cde} )\notag                       \\
     & \quad
    +\mathrm{c.c.}
\end{align}

\subsection{Matching Four-Fermi Interactions}
The low energy effective theory of the light SM fields is given by the
four-fermi Lagrangian, obtained by integrating out the \(W^{\pm}\) and
\(Z\). The result of integrating out the heavy bosons is:
\begin{align}
    \cL_{4F} = -\frac{4G_{F}}{\sqrt{2}}\qty[J^{+}_{\mu}J^{-}_{\mu} + \qty(J^{Z}_{\mu})^{2}]
\end{align}
In the above expression, the charged and neutral currents are given by:
\begin{align}
    J^{+}_{\mu}      & = j^{+}_{\mu}
    + V_{ud}u^{\dagger}\bar{\sigma}_{\mu}d
    + V_{us}u^{\dagger}\bar{\sigma}_{\mu}s
    \\
    J^{-}_{\mu}      & = j^{-}_{\mu}
    + V^{*}_{ud}d^{\dagger}\bar{\sigma}_{\mu}u
    + V^{*}_{us}s^{\dagger}\bar{\sigma}_{\mu}u
    \\
    c_{W}J^{Z}_{\mu} & = c_{W}j^{Z}_{\mu} +
    \sum_{q=u,d,s}\qty(g_{L,q}q^{\dagger}\bar{\sigma}_{\mu}q
    +g_{R,q}\bar{q}^{\dagger}\bar{\sigma}_{\mu}\bar{q})
\end{align}
where \(j^{\pm}_{\mu}(j^{Z}_{\mu})\) are the charged(neutral) currents without light quarks,
\(V_{ij}\) is the CKM matrix and left/right handed couplings are
\begin{align}
    g_{L,u} & = \frac{1}{2} - \frac{2}{3}s_{W}^{2}  &
    g_{L,d} & = -\frac{1}{2} + \frac{1}{3}s_{W}^{2} &
    g_{R,u} & = -\frac{2}{3}s_{W}^{2}               &
    g_{R,d} & = \frac{1}{3}s_{W}^{2}
\end{align}
In terms of the left-handed neutrino gauge eigenstates, the charged and neutral currents
are given by:
\begin{align}
    j^{Z}_{\mu} & =
    \frac{1}{2c_{W}}\hat{\nu}_{i}^{\dagger}\bar{\sigma}_{\mu}\hat{\nu}_{i}
    +\frac{1}{2c_{W}}\qty(-1+2s_{W}^{2})\ell_{i}^{\dagger}\bar{\sigma}_{\mu}\ell_{i}
    -\frac{s_{W}^{2}}{c_{W}}\bar{\ell}_{i}^{\dagger}\bar{\sigma}_{\mu}\bar{\ell}_{i} \\
    j^{+}_{\mu} & =\hat{\nu}_{i}^{\dagger}\bar{\sigma}_{\mu}\ell_{i}
\end{align}
Grouping the left-handed light quarks into a vector \(\bm{q} = \mqty(u & d & s)\)
and the right-handed quarks into
\(\bar{\bm{q}} = \mqty(\bar{u} & \bar{d} & \bar{s})\), we can write the currents
as
\begin{align}
    J^{+}_{\mu}      & = j^{+}_{\mu}
    +
    \bm{q}^{\dagger}\bm{V}\bar{\sigma}_{\mu}\bm{q}
    \\
    J^{-}_{\mu}      & = j^{-}_{\mu}
    + \bm{q}^{\dagger}\bm{V}^{\dagger}\bar{\sigma}_{\mu}\bm{q}
    \\
    c_{W}J^{Z}_{\mu} & = c_{W}j^{Z}_{\mu} +
    \bm{q}^{\dagger}\bm{G}_{L}\bar{\sigma}_{\mu}\bm{q} +
    \bar{\bm{q}}^{\dagger}\bm{G}_{R}\bar{\sigma}_{\mu}\bar{\bm{q}}
\end{align}
where
\begin{align}
    \bm{V}
            & =
    \mqty(0 & V_{ud} & V_{us} \\ 0&0&0\\ 0&0&0),
            &
    \bm{G}_{L,q}
            & =
    \bm{T}_{3,q} - s_{W}^{2}\bm{Q}_{q},
            &
    \bm{G}_{R,q}
            & =
    -s_{W}^{2}\bm{Q}_{q}
\end{align}
with \(\bm{Q}_{q}\) the light-quark charge matrix and \(\bm{T}_{3,q}\) a matrix
containing the light-quark weak-isospin eigenvalues
\begin{align}
    \bm{Q}_{q}
     & =
    \frac{1}{3}\mqty(\dmat{2,-1,-1}),
     &
    \bm{T}_{3,q}
     & =
    \frac{1}{2}\mqty(\dmat{1,-1,-1}),
\end{align}
Expanding out the four-fermi Lagrangian, one finds:
\begin{align}
    %\bm{q}^{\dagger}\bm{V}\bar{\sigma}_{\mu}\bm{q}
    %\bm{q}^{\dagger}\bm{V}^{\dagger}\bar{\sigma}_{\mu}\bm{q}
    %
    %
    -\frac{\sqrt{2}}{4G_{F}}\cL_{4F}
     & =
    \bm{q}^{\dagger}\qty(
    \bm{V}j^{-}_{\mu}
    + \bm{V}^{\dagger}j^{+}_{\mu}
    + \frac{2}{c_{W}}\bm{G}_{L,q}j^{Z}_{\mu}
    )\bar{\sigma}^{\mu}\bm{q}
    +\frac{2}{c_{W}}
    \bar{\bm{q}}^{\dagger}\qty(
    \bm{G}_{R,q}j^{Z}_{\mu}
    )\bar{\sigma}^{\mu}\bar{\bm{q}} \\
     & \quad
    + j^{+}_{\mu}j^{-}_{\mu}
    + j^{Z}_{\mu}j^{Z}_{\mu}\notag  \\
     & \quad
    \qty(\bm{q}^{\dagger}\bm{V}\bar{\sigma}_{\mu}\bm{q})
    \qty(\bm{q}^{\dagger}\bm{V}^{\dagger}\bar{\sigma}_{\mu}\bm{q})
    + \qty(\bm{q}^{\dagger}\bm{G}_{L}\bar{\sigma}_{\mu}\bm{q} +
    \bar{\bm{q}}^{\dagger}\bm{G}_{R}\bar{\sigma}_{\mu}\bar{\bm{q}})^{2}
    \notag
\end{align}
Only the first four terms in the above expression will result in neutrino
interactions (the last two terms contribute to weak interactions among mesons.)
The first two terms are matched onto the left and right handed chiral currents,
resulting in:
\begin{align}
    \cL_{\ChiPT} & \supset \frac{f_{\pi}^{2}}{4}\Tr[
        \qty(D_{\mu}\bm{\Sigma})^{\dagger}
        \qty(D^{\mu}\bm{\Sigma})
    ]
\end{align}
with
\begin{align}
    D_{\mu}\bm{\Sigma}
     & =
    \partial_{\mu}\bm{\Sigma}
    - i\bm{R}_{\mu}\bm{\Sigma}
    + i\bm{\Sigma}\bm{L}_{\mu}, \\
    \bm{R}_{\mu}
     & =
    \frac{2}{c_{W}}
    \bm{G}_{R,q}j^{Z}_{\mu},
     &
    \bm{L}_{\mu}
     & =
    \bm{V}j^{-}_{\mu}
    + \bm{V}^{\dagger}j^{+}_{\mu}
    + \frac{2}{c_{W}}\bm{G}_{L,q}j^{Z}_{\mu}
\end{align}
Note that we can decompose the currents into Gell-Mann matrices, yielding:
\begin{align}
    \bm{L}_{\mu}
     & =
    -\frac{1}{3c_{W}}j^{Z}_{\mu}\bm{I}
    +\frac{2(1-s_{W}^{2})}{c_{W}}\qty(\bm{\lambda}_{3}+\frac{1}{\sqrt{3}}\bm{\lambda}_{8})j^{Z}_{\mu}
    +
    \qty[
    \qty(
    V^{*}_{ud}\bm{\lambda}^{+}_{12} + V^{*}_{us}\bm{\lambda}^{+}_{45}
    )j^{+}_{\mu}
    +\mathrm{c.c.}
    ]\notag \\
    \bm{R}_{\mu}
     & =
    -\frac{2s_{W}^{2}}{c_{W}^{2}}
    \qty(\bm{\lambda}_{3}+\frac{1}{\sqrt{3}}\bm{\lambda}_{8})j^{Z}_{\mu}
\end{align}
where \(\bm{\lambda}^{\pm}_{12} = \bm{\lambda}_{1} \mp i\bm{\lambda}_{2}\) and
\(\bm{\lambda}^{\pm}_{45} = \bm{\lambda}_{4} \mp i\bm{\lambda}_{5}\).
The Lagrangian containing currents and mesons can be brought into the following
form:
\begin{align}
    \cL & =
    -\frac{4G_{F}}{\sqrt{2}}\qty(
    j^{Z}_{\mu}\cJ^{0}_{\mu}
    + \qty(j^{+}_{\mu}\cJ^{+}_{0} + \mathrm{c.c.})
    +\qty(j^{Z}_{\mu})^{2}\cS^{0}
    +j^{Z}_{\mu}\qty(j^{+}_{\mu}\cS^{+}+\mathrm{c.c.})
    )
\end{align}
Here, the neutral meson current \(\cJ^{0}_{\mu}\) is given by:
\begin{align}
    \cJ^{0}_{\mu} & =
    \frac{f_{\pi}}{c_{W}}\qty[
        \partial^{\mu}\pi^{0}
        + \frac{1}{\sqrt{3}}
        \partial^{\mu}\eta
    ]
    - \frac{i (1-2s_{W}^{2})}{c_{W}}
    \qty[
    \pi^{+}\overleftrightarrow{\partial}_{\mu}\pi^{-} +
    K^{+}\overleftrightarrow{\partial}_{\mu}K^{-}
    ]
\end{align}
where \(X\overleftrightarrow{\partial}_{\mu}Y \equiv X\partial_{\mu}Y - Y\partial_{\mu}X\).
The charged meson current is:
\begin{align}
    \cJ^{+}_{\mu}
     & =
    \frac{f_{\pi}}{\sqrt{2}}\qty[
    V^{*}_{ud}\partial^{\mu}\pi^{+}
    + V^{*}_{us}\partial^{\mu}K^{+}
    ]
    \\
     & \quad
    + i
    \frac{V^{*}_{ud}}{\sqrt{2}}\qty(
    \bar{K}^{0}\overleftrightarrow{\partial}_{\mu}K^{+}
    + \sqrt{2}\pi^{+}\overleftrightarrow{\partial}_{\mu}\pi^{0}
    )\notag  \\
     & \quad
    +i\frac{V_{us}^{*}}{2}\qty(
    K^{0}\overleftrightarrow{\partial}_{\mu}\pi^{+}
    +\sqrt{\frac{3}{2}}K^{+}\overleftrightarrow{\partial}_{\mu}\eta
    +\frac{1}{\sqrt{2}}K^{+}\overleftrightarrow{\partial}_{\mu}\pi^{0}
    )\notag
\end{align}
The neutral meson density \(\cS_{0}\) is
\begin{align}
    \cS^{0} & =
    - \frac{4(1-s_{W}^{2})s_{W}^{2}}{c_{W}^{2}}
    \qty[
    \pi^{+}\pi^{-} +
    K^{+}K^{-}
    ]
\end{align}
and the charged meson density \(\cS_{+}\) is
\begin{align}
    \cS^{+} & =
    \frac{s_{W}^{2}}{c_{W}}\qty(
    V^{*}_{ud}\qty(
    \sqrt{2}\pi^{+}\pi^{0}
    - K^{+}\bar{K}^{0}
    )
    +V^{*}_{us}\qty(
    \sqrt{\frac{3}{2}}K^{+}\eta
    + \frac{1}{\sqrt{2}}K^{+}\pi^{0}
    - \pi^{+}K^{0}
    )
    )
\end{align}
