# Supplementary material for: Sterile Neutrinos from Dark Matter: A $\nu$ Nightmare?
Source: arXiv:2211.05996 source file (2022-11-11)
Supplement: Supplementary file 3 [file appendix_general_rhneutrino.tex]

\section{General RHN Model}

In this paper, we considered simplified cases where we assumed that the RHN of interest mixes with a single SM neutrino flavor, without considering the details of neutrino masses and mixings. In this appendix, we discuss such details for completeness.

Consider a theory with \(n\) right-handed neutrinos \(\hat{\rhn}_1, \dots, \hat{\rhn}_n\) that
interact with the standard model through a Yukawa interaction. The general
renormalizable Lagrangian for this theory is
\begin{align}\label{eqn:GeneralRHN}
	\mathcal{L}\supset
	\hat{\rhn}_i^{\dagger}\bar{\sigma}_{\mu}\partial^{\mu}\hat{\rhn}_i
	-\frac{1}{2}\qty(\hat{\bm{m}}^{ij}\hat{\rhn}_i\hat{\rhn}_j + \mathrm{c.c.})
	+ \qty(\Phi_{a}\epsilon^{ab}\hat{L}_{b,i}\bm{Y}^{ij}_{\nu}\hat{\rhn}_{j}
	- \Phi_{a}^{\dagger}\hat{L}_{a,i}\bm{Y}^{ij}_{\ell}\hat{\bar{\ell}}_{j} + \mathrm{c.c})
\end{align}
where \(\hat{\bm{m}}\) is an \(n\times n\) complex symmetric matrix, and
\(\bm{Y}_{\nu}\) is a \(3\times n\) complex matrix. Here \(\Phi\) is the Higgs doublet
\begin{align}
	\Phi = \frac{1}{\sqrt{2}}\mqty(\sqrt{2}G^{+} \\ v + h + iG^{0})
\end{align}
with \(v = 246 \ \mathrm{GeV}\) being the Higgs vacuum expectation value, \(h\)
the Higgs and \(G^{+},G^{0}\) the changed and neutral Goldstones. The lepton
doublet is parameterized as:
\begin{align}
	\hat{L}_{i} = \mqty(\hat{\nu}_i \\ \hat{\ell}_i)
\end{align}
with \(i\in\qty{1,2,3}\). \(\hat{\nu}_i\) are the left-handed neutrinos and
\(\ell_i\) are the gauge eigenstates of the charged leptons.

\subsection{Mass Diagonalization}
%\subsubsection{Exact Mass Diagonalization}
Expanding out \ref{eqn:GeneralRHN}, the mass terms for the neutrinos are:
\begin{align}\label{eqn:RHNMass}
	\cL_{\nu,\mathrm{mass}}\supset
	-\frac{1}{2}\qty(\hat{\bm{m}}^{ij}\hat{\rhn}_i\hat{\rhn}_j + \mathrm{c.c.})
	- \frac{v}{\sqrt{2}}\qty(\hat{\nu}_{i}\bm{Y}^{ij}_{\nu}\hat{\rhn}_{j} + \mathrm{c.c})
\end{align}
Gathering the left- and right-handed neutrinos into a vector
\begin{align}
	\hat{\cN} = \mqty(\hat{\nu}_1 & \hat{\nu}_2 & \hat{\nu}_3 & \hat{\rhn}_1 & \cdots & \hat{\rhn}_n)^{T}
\end{align}
we can write the mass terms as:
\begin{align}\label{eqn:RHNMassMatrix}
	\cL_{\nu,\mathrm{mass}}
	                  & \supset
	-\frac{1}{2}\hat{\cN}_{i}\bm{M}^{ij}\hat{\cN}_j,
	                  &
	\hat{\bm{M}}      & = \mqty(
	\bm{0}_{3\times3} & \hat{\bm{m}}_{D} \\
	\hat{\bm{m}}_{D}  & \hat{\bm{m}}
	)
\end{align}
where \(\hat{\bm{m}}_{D} = v\bm{Y}_{\nu}/\sqrt{2}\). The neutrino mass matrix is diagonalized
using Takagi diagonalization with a unitary matrix \(\bm{\Omega}\). The diagonalization condition
is
\begin{align}\label{eqn:DiagCond}
	\bm{\Omega}^{T}\hat{\bm{M}}\bm{\Omega} & = m^{i}_{\nu}\delta_{ij}, &  & (\text{no sum over } i)
\end{align}
where \(m^{i}_{\nu}\) are the masses of the neutrino mass eigenstates. It is convinient to
write \(\bm{\Omega}\) as
\begin{align}\label{eqn:OmegaDef}
	\bm{\Omega} & = \mqty(\OmegaVVb & \OmegaVNb \\ \OmegaNVb & \OmegaNNb)
\end{align}
where \(\OmegaVVb\) is a \(3\times3\) matrix, \(\OmegaVNb\) is a \(3\times n\) matrix,
\(\OmegaNVb\) is a \(n\times3\) matrix and \(\OmegaNNb\) is a \(n\times n\) matrix.
The neutrino eigenstates are related to the gauge eigenstates through:
\begin{align}
	\hat{\nu}_{i}  & = \qty(\OmegaVVb)^{ij}\nu_j + \qty(\OmegaVNb)^{ij}\rhn_j \\
	\hat{\rhn}_{i} & = \qty(\OmegaNVb)^{ij}\nu_j + \qty(\OmegaNNb)^{ij}\rhn_j
\end{align}
By \ref{eqn:DiagCond}, we find that the block matrices satisfy the following conditions:
\begin{align}
	\bm{m}_{\nu}       & =
	\OmegaVVb^{T}\hat{\bm{m}}_{D}\OmegaNVb+\OmegaNVb^{T}\hat{\bm{m}}^{T}_{D}\OmegaVVb+\OmegaNVb^{T}\hat{\bm{m}}\OmegaNVb \\
	\bm{0}_{3\times n} & =
	\OmegaNVb^{T}\hat{\bm{m}}^{T}_{D}\OmegaVNb+\OmegaVVb^{T}\hat{\bm{m}}_{D}\OmegaNNb+\OmegaNVb^{T}\hat{\bm{m}}\OmegaNNb \\
	\bm{0}_{n\times 3} & =
	\OmegaVNb^{T}\hat{\bm{m}}_{D}\OmegaNVb
	+\OmegaNNb^{T}\hat{\bm{m}}^{T}_{D}\OmegaVVb
	+\OmegaNNb^{T} \hat{\bm{m}}\OmegaNVb                                                                                 \\
	\bm{m}_{\rhn}      & =
	\OmegaVNb^{T}\hat{\bm{m}}_{D}\OmegaNNb
	+\OmegaNNb^{T}\hat{\bm{m}}^{T}_{D}\OmegaVNb
	+\OmegaNNb^{T} \hat{\bm{m}}\OmegaNNb
\end{align}
where \(\bm{m}_{\nu}\) is a diagonal \(3\times3\) mass matrix and \(\bm{m}_{\rhn}\) is a
\(n\times n\) diagonal mass matrix. These conditions can be flipped to obtain \(\hat{\bm{m}}_{D}\) and \(\hat{\bm{m}}\)
in terms of the mixing and mass matrices:
\begin{align}
	\hat{\bm{m}}_{D}  & = \OmegaVVb^{*}\bm{m}_{\nu}\OmegaNVb^{\dagger} + \OmegaVNb^{*}\bm{m}_{\rhn}\OmegaNNb^{\dagger} \\
	\hat{\bm{m}}      & = \OmegaNVb^{*}\bm{m}_{\nu}\OmegaNVb^{\dagger} + \OmegaNNb^{*}\bm{m}_{\rhn}\OmegaNNb^{\dagger} \\
	\bm{0}_{3\times3} & = \OmegaVVb^{*}\bm{m}_{\nu}\OmegaVVb^{\dagger} + \OmegaVNb^{*}\bm{m}_{\rhn}\OmegaVNb^{\dagger}
\end{align}

By unitarity, we have:
\begin{align}
	\bm{1}_{3\times3}  & = \OmegaVVb^{\dagger}\OmegaVVb+\OmegaVNb^{\dagger}\OmegaNVb \\
	\bm{0}_{3\times n} & = \OmegaVVb^{\dagger}\OmegaVNb+\OmegaNVb^{\dagger}\OmegaNNb \\
	\bm{0}_{n\times3}  & = \OmegaVNb^{\dagger}\OmegaVVb+\OmegaNNb^{\dagger}\OmegaNVb \\
	\bm{1}_{n\times n} & = \OmegaNVb^{\dagger}\OmegaVNb+\OmegaNNb^{\dagger}\OmegaNNb
\end{align}

The charged lepton mass matrix is diagonalized in a slightly different fashion (since the mass matrix
is no longer a complex symmetric matrix), which we review here. The charge lepton
yukawa interaction yields the following mass terms:
\begin{align}
	\cL_{\ell,\mathrm{mass}}\supset -\frac{v}{\sqrt{2}}\bm{Y}_{\ell}^{ij}
	\hat{\ell}_{i}\hat{\bar{\ell}}_{j} + \mathrm{c.c.}
\end{align}
where \(\hat{\bar{\ell}}_{i}\) is the gauge eigenstate for the right-handed charged leptons.
To diagonalize \(v\bm{Y}_{\ell}/\sqrt{2}\), we employ singular-value decomposition. Apply
a unitary matrix \(\bm{L}_{\ell}\) and \(\bm{R}_{\ell}\) to the left-handed and right-handed
charged leptons, respectively. Then, we require that:
\begin{align}
	\frac{v}{\sqrt{2}}
	\qty(\bm{L}^T\bm{Y}_{\ell}\bm{R})^{ij}
	= m_{i}\delta_{ij}
	(\text{no sum over } i)
\end{align}
The masses \(m_{i}\) can be obtained by compute the positive square roots of
\(\bm{Y}_{\ell}^{\dagger}\bm{Y}_{\ell}\) (which is a Hermitian matrix.) From now on,
we will assume that the charge leptons rotations have been performed. We will also rotate
the left-handed neutrinos by \(\bm{L}_{\ell}\) and redefine the neutrino Yukawa such
that \(\bm{Y}_{\nu}\to \bm{L}_{\ell}\bm{Y}_{\nu}\).

%\subsubsection{Approximate Mass Diagonalization}
%\input{files/appendix/general_rhn/mass_diag_approx.tex}

\subsection{Interactions}
First, we consider the kinetic term for the lepton doublet:
\begin{align}
	L^{\dagger}_{a,i}\bar{\sigma}_{\mu}D^{\mu}L_{a,i} =
	\frac{e}{\sqrt{2}s_{W}}W^{-}_{\mu}\ell_{i}^{\dagger}\bar{\sigma}^{\mu}\hat{\nu}_{i}
	+\frac{e}{\sqrt{2}s_{W}}W^{+}_{\mu}\hat{\nu}_{i}^{\dagger}\bar{\sigma}^{\mu}\ell_{i}
	-\frac{e}{2c_{W}s_{W}}Z_{\mu}\hat{\nu}_{i}^{\dagger}\bar{\sigma}^{\mu}\hat{\nu}_{i} + \cdots
\end{align}
Rotating the neutrinos, we find
\begin{align}
	L^{\dagger}_{a,i}\bar{\sigma}_{\mu}D^{\mu}L_{a,i}
	 & = \cdots
	%----------
	+\frac{e}{\sqrt{2}s_{W}}W^{-}_{\mu}\ell_{i}^{\dagger}\bar{\sigma}^{\mu}
	\qty(\OmegaVVb)^{ij}\nu_{j}
	+\frac{e}{\sqrt{2}s_{W}}W^{-}_{\mu}\ell_{i}^{\dagger}\bar{\sigma}^{\mu}
	\qty(\OmegaVNb)^{ij}\rhn_{j}\notag                                                                                    \\
	%----------
	 & \quad
	+\frac{e}{\sqrt{2}s_{W}}W^{+}_{\mu}\nu_{i}^{\dagger}
	\qty(\OmegaVVb^{\dagger})^{ij}\bar{\sigma}^{\mu}\ell_{j}
	+\frac{e}{\sqrt{2}s_{W}}W^{+}_{\mu}\rhn_{i}^{\dagger}
	\qty(\OmegaVNb^{\dagger})^{ij}\bar{\sigma}^{\mu}\ell_{j}\notag                                                        \\
	%----------
	 & \quad
	+\frac{e}{2c_{W}s_{W}}Z_{\mu}\nu_{i}^{\dagger}\qty(\OmegaVVb^{\dagger}\OmegaVVb)^{in}\bar{\sigma}^{\mu}\nu_{j}
	+\frac{e}{2c_{W}s_{W}}Z_{\mu}\nu_{i}^{\dagger}\qty(\OmegaVVb^{\dagger}\OmegaVNb)^{in}\bar{\sigma}^{\mu}\rhn_{j}\notag \\
	%----------
	 & \quad
	+\frac{e}{2c_{W}s_{W}}Z_{\mu}\rhn_{n}^{\dagger}\qty(\OmegaVNb^{\dagger}\OmegaVVb)^{ij}\bar{\sigma}^{\mu}\nu_{j}
	+\frac{e}{2c_{W}s_{W}}Z_{\mu}\rhn_{n}^{\dagger}\qty(\OmegaVNb^{\dagger}\OmegaVNb)^{ij}\bar{\sigma}^{\mu}\rhn_{j}\notag
	%----------
\end{align}
Written in this way, we can interpret parts of mixing matrix. From the first two terms, we identify
\(\OmegaVVb\) as the PMNS matrix and
\(\OmegaVNb\) and its right-handed partner. We will now rename
\(\OmegaVVb\) as \(\bm{\cK}_{L}\) and
\(\OmegaVNb\) as \(\bm{\cK}_{R}\). Then, the above can be
written as
\begin{align}
	% \qty(\OmegaVVb)^{ij}\nu_{j} + \qty(\OmegaVNb)^{ij}\rhn_{j}
	% \qty(\OmegaNVb)^{ij}\nu_{j} + \qty(\OmegaNNb)^{ij}\rhn_{j}
	L^{\dagger}_{a,i}\bar{\sigma}_{\mu}D^{\mu}L_{a,i}
	 & = \cdots
	%----------
	+\frac{e}{\sqrt{2}s_{W}}W^{-}_{\mu}\ell_{i}^{\dagger}\bar{\sigma}^{\mu}\qty(\bm{\cK}_{L})^{ij}\nu_{j}
	+\frac{e}{\sqrt{2}s_{W}}W^{-}_{\mu}\ell_{i}^{\dagger}\bar{\sigma}^{\mu}\qty(\bm{\cK}_{R})^{ij}\rhn_{j}\notag                \\
	%----------
	 & \quad
	+\frac{e}{\sqrt{2}s_{W}}W^{+}_{\mu}\nu_{i}^{\dagger}\qty(\bm{\cK}_{L}^{\dagger})^{ij}\bar{\sigma}^{\mu}\ell_{j}
	+\frac{e}{\sqrt{2}s_{W}}W^{+}_{\mu}\rhn_{i}^{\dagger}\qty(\bm{\cK}_{R}^{\dagger})^{ij}\bar{\sigma}^{\mu}\ell_{j}\notag      \\
	%----------
	 & \quad
	+\frac{e}{2c_{W}s_{W}}Z_{\mu}\nu_{i}^{\dagger}\qty(\bm{\cK}_{L}^{\dagger}\bm{\cK}_{L})^{ij}\bar{\sigma}^{\mu}\nu_{j}
	+\frac{e}{2c_{W}s_{W}}Z_{\mu}\nu_{i}^{\dagger}\qty(\bm{\cK}_{L}^{\dagger}\bm{\cK}_{R})^{ij}\bar{\sigma}^{\mu}\rhn_{j}\notag \\
	%----------
	 & \quad
	+\frac{e}{2c_{W}s_{W}}Z_{\mu}\rhn_{i}^{\dagger}\qty(\bm{\cK}_{R}^{\dagger}\bm{\cK}_{L})^{ij}\bar{\sigma}^{\mu}\nu_{j}
	+\frac{e}{2c_{W}s_{W}}Z_{\mu}\rhn_{i}^{\dagger}\qty(\bm{\cK}_{R}^{\dagger}\bm{\cK}_{R})^{ij}\bar{\sigma}^{\mu}\rhn_{j}\notag
	%----------
\end{align}
Expanding out the Yukawa term in Eqn.~(\ref{eqn:GeneralRHN}), we find:
\begin{align}
	\Phi_{a}\epsilon^{ab}\hat{L}_{b,i}\bm{Y}^{ij}_{\nu}\hat{\rhn}_{j}
	 & =
	\frac{2}{v}G^{+}\ell_{i}\qty(\hat{\bm{m}})^{ij}_{D}\hat{\rhn}_j +
	\frac{1}{v}(h + iG^{0})\hat{\nu}_i\hat{\bm{m}}^{ij}_{D}\hat{\rhn}_{j}
	+ \frac{1}{v}\hat{\nu}_i\hat{\bm{m}}^{ij}_{D}\hat{\rhn}_{j} \\
	-\Phi_{a}^{\dagger}\hat{L}_{a,i}\bm{Y}^{ij}_{\ell}\hat{\bar{\ell}}_{j}
	 & =
	-\frac{\sqrt{2}}{v}G^{-}m_{\ell_{i}}\bar{\ell}_{i}\hat{\nu}_{i} +\cdots
\end{align}
Rotating the neutrinos, and using:
\begin{align}
	\hat{\bm{m}}_{D}\OmegaNVb & = \bm{\cK}_{L}^{*}\bm{m}_{\nu}, & %  \\
	\hat{\bm{m}}_{D}\OmegaNNb & = \bm{\cK}_{R}^{*}\bm{m}_{\rhn}   %                                                                                   \\
	%\OmegaNVb^{T}\hat{\bm{m}}\OmegaNVb & = \bm{m}_{\nu} - \bm{\cK}_{L}^{T}\bm{\cK}_{L}^{*}\bm{m}_{\nu} - \bm{m}_{\nu}\bm{\cK}_{L}^{\dagger}\bm{\cK}_{L}    \\
	%\OmegaNVb^{T}\hat{\bm{m}}\OmegaNNb & = -\bm{\cK}_{L}^{T}\bm{\cK}_{R}^{*}\bm{m}_{\rhn} - \bm{m}_{\nu}\bm{\cK}_{L}^{\dagger}\bm{\cK}_{R}                 \\
	%\OmegaNNb^{T}\hat{\bm{m}}\OmegaNNb & = \bm{m}_{\rhn} - \bm{\cK}_{R}^{T}\bm{\cK}_{R}^{*}\bm{m}_{\rhn} - \bm{m}_{\rhn}\bm{\cK}_{R}^{\dagger}\bm{\cK}_{R}
\end{align}
we find the following
\begin{align}
	\Phi_{a}\epsilon^{ab}\hat{L}_{b,i}\bm{Y}^{ij}_{\nu}\hat{\rhn}_{j} =
	%-----------------------------------------------------------
	 & \quad
	\frac{\sqrt{2}}{v}G^{+}\ell_{i}{\qty(\bm{\cK}_{L}^{*}\bm{m}_{\nu})}^{ij}\nu_{j}
	+ \frac{\sqrt{2}}{v}G^{+}\ell_{i}{\qty(\bm{\cK}_{R}^{*}\bm{m}_{\nu})}^{ij}\rhn_{j}
	\\
	%-----------------------------------------------------------
	 & \quad
	- \frac{h+iG^{0}}{v}\nu_i\qty(
	\bm{\cK}_{L}^{T}\bm{\cK}_{L}^{*}\bm{m}_{\nu}
	)^{ij}\nu_{j}
	- \frac{h+iG^{0}}{v}\rhn_i\qty(
	\bm{\cK}_{R}^{T}\bm{\cK}_{R}^{*}\bm{m}_{\rhn}
	)^{ij}\rhn_{j}
	\notag   \\
	%-----------------------------------------------------------
	 & \quad
	- \frac{h+iG^{0}}{v}\nu_i\qty(
	\bm{\cK}_{L}^{T}\bm{\cK}_{R}^{*}\bm{m}_{\rhn}
	)^{ij}\rhn_{j}
	- \frac{h+iG^{0}}{v}\rhn_i\qty(
	\bm{\cK}_{R}^{T}\bm{\cK}_{L}^{*}\bm{m}_{\nu}
	)^{ij}\nu_{j}
	\notag
\end{align}
The interactions with the right-handed charged leptons are:
\begin{align}
	-\Phi_{a}^{\dagger}\hat{L}_{a,i}\bm{Y}^{ij}_{\ell}\hat{\bar{\ell}}_{j}
	 & =
	-\frac{\sqrt{2}}{v}G^{-}\qty(\bm{m}_{\ell}\bm{\cK}_{L})^{ij}\bar{\ell}_{i}\nu_{j}
	-\frac{\sqrt{2}}{v}G^{-}\qty(\bm{m}_{\ell}\bm{\cK}_{R})^{ij}\bar{\ell}_{i}\rhn_{j}
\end{align}

\input{files/appendix/general_rhn/feynman_rules/w_ll_v.tex}
\input{files/appendix/general_rhn/feynman_rules/z_v_v.tex}
\input{files/appendix/general_rhn/feynman_rules/g_ll_v.tex}
\input{files/appendix/general_rhn/feynman_rules/g_lr_v.tex}
\input{files/appendix/general_rhn/feynman_rules/h_v_v.tex}
\input{files/appendix/general_rhn/feynman_rules/g_v_v.tex}

\subsection{Single RH Neutrino}

Here we specialize the above discussion to the case with a single RH neutrino (i.e
\(n=1\)). In this case, the neutrino mass matrix takes the form
\begin{align}
	\hat{\bm{M}} = \mqty(
	0             & 0               & 0                & \hat{m}_{D,e}    \\
	0             & 0               & 0                & \hat{m}_{D,\mu}  \\
	0             & 0               & 0                & \hat{m}_{D,\tau} \\
	\hat{m}_{D,e} & \hat{m}_{D,\mu} & \hat{m}_{D,\tau} & \mu              \\
	)
\end{align}
where \(\hat{m}_{D,\ell} = v y_{\ell}/\sqrt{2}\). For now, we assume the \(\hat{m}_{D,\ell}\)
are real (we relax this later.) The eigenvalues of
\(\hat{\bm{M}}\) are:
\begin{align}
	m_{1} & = m_{2} = 0                                     \\
	m_{3} & = \frac{\mu}{2}\qty(\sqrt{1 + 2\epsilon^{2}}-1) \\
	m_{4} & = \frac{\mu}{2}\qty(\sqrt{1 + 2\epsilon^{2}}+1)
\end{align}
where \(\epsilon=vy/\mu\) and \(y^{2}=y_{e}^{2}+y_{\mu}^{2}+y_{\tau}^{2}\).
Then mass eigenstates are:
\begin{align}
	\nu_{1} & = \frac{1}{\sqrt{y^{2}_{e}\qty(y^{2}_{\mu} + y^{2}_{\tau})}}
	\mqty(0                                                                               \\
	-y_{e}y_{\tau}                                                                        \\
	y_{e}y_{\mu}                                                                          \\
	0),     &
	\nu_{2} & = \frac{1}{\sqrt{y^{2}y_{\tau}^2y_{\mu}^{2}\qty(y_{\mu}^{2}+y_{\tau}^{2})}}
	\mqty(
	-y_{\mu}y_{\tau}\qty(y_{\mu}^{2}+y_{\tau}^{2})                                        \\
	y_{e}y^{2}_{\mu}y_{\tau}                                                              \\
	y_{e}y_{\mu}y^{2}_{\tau}                                                              \\
	0)                                                                                    \\
	\nu_{3} & = \frac{i}{\sqrt{2m^{2}_{3} + v^2y^2}}
	\mqty(
	v y_{e}                                                                               \\
	v y_{\mu}                                                                             \\
	v y_{\tau}                                                                            \\
	-\sqrt{2}m_{3}
	),      &
	\nu_{4} & = \frac{1}{\sqrt{2m^{2}_{4} + v^2y^2}}
	\mqty(
	v y_{e}                                                                               \\
	v y_{\mu}                                                                             \\
	v y_{\tau}                                                                            \\
	-\sqrt{2}m_{4}
	)
\end{align}
with \(\Omega\) being the matrix with the eigenstates as columns. If we set
\(y_{\tau} = y\) and \(y_{e}=y_{\mu}=0\), we \(\Omega\) is (which we will denote
as \(\Omega_{0}\))
\begin{align}
	\Omega_{0}
	  & =
	\mqty(
	1 & 0 & 0                            & 0                           \\
	0 & 1 & 0                            & 0                           \\
	0 & 0 & i\sqrt{\frac{m_4}{m_4+m_3}}  & \sqrt{\frac{m_3}{m_4+m_3}}  \\
	0 & 0 & -i\sqrt{\frac{m_3}{m_4+m_3}} & \sqrt{\frac{m_4}{m_4+m_3}})
\end{align}
If we define a mixing angle \(\theta\) such that:
\begin{align}
	\cos\theta & = \sqrt{\frac{m_4}{m_4+m_3}}, &
	\sin\theta & = \sqrt{\frac{m_3}{m_4+m_3}}
\end{align}
then \(\tan^2\theta = m_{3}/m_{4}\). We can therefore define all the parameters in
terms of the mixing angle and the heavy mass. Let \(m_{\nu}=m_{3}\) and
\(m_{4} = m_{\rhn}\). Then,
\begin{align}
	m_{\nu} & = m_{\rhn}\tan^2\theta,                 &
	y       & = \frac{\sqrt{2}m_{\rhn}}{v}\tan\theta, &
	\mu     & = m_{\rhn}\qty(1-\tan^2\theta)
\end{align}
In the case where \(y_{e},y_{\mu}\) and \(y_{\tau}\) are all non-zero, then we
first perform a rotation such that we remove \(y_{e}\) and \(y_{\mu}\). This is
done using a rotation matrix \(R\) such that:
\begin{align}
	R^{T}\hat{\bm{M}}R =
	\mqty(
	0 & 0 & 0                  & 0                  \\
	0 & 0 & 0                  & 0                  \\
	0 & 0 & 0                  & \sqrt{v}y/\sqrt{2} \\
	0 & 0 & \sqrt{v}y/\sqrt{2} & \mu                \\
	)
\end{align}
To achive this, we use the following rotation matrix:
\begin{align}
	R = \mqty(
	\cos\alpha\cos\beta & -\sin\beta & \cos\beta\sin\alpha & 0 \\
	\cos\alpha\sin\beta & \cos\beta  & \sin\alpha\sin\beta & 0 \\
	-\sin\alpha         & 0          & \cos\alpha          & 0 \\
	0                   & 0          & 0                   & 1
	)
\end{align}
where \(\alpha\) and \(\beta\) are such that
\begin{align}
	y_{e}    & = y\cos\beta\sin\alpha, &
	y_{\mu}  & = y\sin\beta\sin\alpha, &
	y_{\tau} & = y\cos\alpha,          &
\end{align}
Then, \(R^{T}\hat{\bm{M}}R\) is diagonalized using the above \(\Omega_{0}\). That
is, \(\Omega^{T}_{0}R^{T}\hat{\bm{M}}R\Omega_{0}\) is diagonal. And therefore, we
identify the full roation matrix as \(\Omega = R\Omega_{0}\), which is:
\begin{align}
	\Omega = \mqty(
	\cos\alpha\cos\beta & -\sin\beta & i \sin\alpha\cos\beta\cos\theta & \sin\alpha\cos\beta\sin\theta \\
	\cos\alpha\sin\beta & \cos\beta  & i \sin\alpha\sin\beta\cos\theta & \sin\alpha\sin\beta\sin\theta \\
	-\sin\alpha         & 0          & i \cos\alpha\cos\theta          & \cos\alpha\sin\theta          \\
	0                   & 0          & -i \sin\theta                   & \cos\theta                    \\
	)
\end{align}

Lastly, we let the \(y_{\ell}\) be complex. In this case, we need to remove the
phases before applying the above \(\Omega\). We can write
\(\tilde{y}_{\ell}= y_{\ell}e^{i\delta_{\ell}}\). We can rephase the RH-Neutrino field
to absorb the phase of \(\mu\). Thus, the mass matrix with complex Yukawas is:
\begin{align}
	\hat{\bm{M}} = \frac{v}{\sqrt{2}}\mqty(
	0             & 0               & 0                & \tilde{y}_{e}    \\
	0             & 0               & 0                & \tilde{y}_{\mu}  \\
	0             & 0               & 0                & \tilde{y}_{\tau} \\
	\tilde{y}_{e} & \tilde{y}_{\mu} & \tilde{y}_{\tau} & \sqrt{2}\mu/v    \\
	)
\end{align}
Applying a phase matrix \(\bm{P}\) to the mass matrix as \(\bm{P}^{T}\hat{\bm{M}}\bm{P}\)
removes all of the phases. Here, the matrix \(\bm{P}\) is given by:
\begin{align}
	\bm{P}
	=
	\mqty(\dmat{
		e^{-i\delta_{e}} ,
		e^{-i\delta_{\mu}},
		e^{-i\delta_{\tau}},
		1
	})
\end{align}
Thus, the full mixing matrix \(\Omega\) for the neutrinos is given by the following product of
rotations and phases:
\begin{align}
	\Omega      & =
	\mqty(\dmat{
		e^{-i\delta_{e}} ,
		e^{-i\delta_{\mu}},
		e^{-i\delta_{\tau}},
		1
	})
	\mqty(
	\dmat{
	\cos\beta   & -\sin\beta                   \\
	\sin\beta   & \cos\beta,1,1}
	)                                          \\
	            & \quad\times
	\mqty(\dmat{
	\cos\alpha  &                & \sin\alpha  \\
	            & 1              &             \\
	-\sin\alpha &                & \cos\alpha,
		1
	})
	\mqty(\dmat{
		1,1,
	\cos\theta  & \sin\theta                   \\
	-\sin\theta & \cos\theta                   \\
	})
	\mqty(\dmat{1,1,e^{i\pi/2},1})
\end{align}
If we take the 3 angles and the heavy neutrino mass as our parameters, the
yukawas and majorana mass are given by:
\begin{align}
	\tilde{y}_{e}    & =\frac{\sqrt{2}m_{\rhn}}{v}\tan\theta\cos\beta\sin\alpha e^{i\delta_{e}},   &
	\tilde{y}_{\mu}  & =\frac{\sqrt{2}m_{\rhn}}{v}\tan\theta\sin\beta\sin\alpha e^{i\delta_{\mu}},   \\
	\tilde{y}_{\tau} & =\frac{\sqrt{2}m_{\rhn}}{v}\tan\theta\cos\alpha e^{i\delta_{\tau}},         &
	\mu              & = m_{\rhn}(1-\tan^2\theta)
\end{align}
and the light neutrino mass is \(m_{\nu} = m_{\rhn}\tan^2\theta\). Additionally, the
PMNS matrices are:
\begin{align}
	\bm{\cK}_{L}
	                                      &
	=
	\mqty(
	e^{-i\delta_{e}}\cos\alpha\cos\beta   &
	-e^{-i\delta_{e}}\sin\beta            &
	i \sin\alpha\cos\beta\cos\theta                   \\
	%e^{-i\delta_{e}}\sin\alpha\cos\beta\sin\theta                             \\
	%----
	e^{-i\delta_{\mu}}\cos\alpha\sin\beta &
	e^{-i\delta_{\mu}}\cos\beta           &
	i e^{-i\delta_{\mu}}\sin\alpha\sin\beta\cos\theta \\
	%& e^{-i\delta_{\mu}}\sin\alpha\sin\beta\sin\theta \\
	%----
	-e^{-i\delta_{\tau}}\sin\alpha        &
	0                                     &
	i e^{-i\delta_{\tau}}\cos\alpha\cos\theta
	%& \cos\alpha\sin\theta          \\
	)                                                 \\
	\bm{\cK}_{R}
	                                      &
	=
	\mqty(
	%e^{-i\delta_{e}}\cos\alpha\cos\beta   &
	%-e^{-i\delta_{e}}\sin\beta            &
	%i \sin\alpha\cos\beta\cos\theta                   \\
	e^{-i\delta_{e}}\sin\alpha\cos\beta\sin\theta     \\
	%----
	%e^{-i\delta_{\mu}}\cos\alpha\sin\beta &
	%e^{-i\delta_{\mu}}\cos\beta           &
	%i e^{-i\delta_{\mu}}\sin\alpha\sin\beta\cos\theta \\
	e^{-i\delta_{\mu}}\sin\alpha\sin\beta\sin\theta   \\
	%----
	%-e^{-i\delta_{\tau}}\sin\alpha        &
	%0                                     &
	%i e^{-i\delta_{\tau}}\cos\alpha\cos\theta
	\cos\alpha\sin\theta                              \\
	)
\end{align}

In the above parameterization, we can see that cases of the RH-neutrino mixing with only
a single LH-neutrino are:
\begin{align}
	\text{electron} & : & \beta & =0,                 & \alpha & =\pi/2, \\
	\text{muon}     & : & \beta & =\pi/2,             & \alpha & =\pi/2, \\
	\text{tau}      & : & \beta & =\mathrm{anything}, & \alpha & =0
\end{align}
