# Supplementary material for: Sterile Neutrinos from Dark Matter: A $\nu$ Nightmare?
Source: arXiv:2211.05996 source file (2022-11-11)
Supplement: Supplementary file 4 [file appendix_partial_widths.tex]

\section{Right-Handed Neutrino Partial Widths}

\subsection{Two-Body Partial Widths}
Here we compute the partial widths of the general RH neutrino model. First, we
compute the widths for right-handed neutrinos, decaying into a Higgs, Z-boson and
W-boson. We will then compute the widths into meson final states.

\subsubsection{\texorpdfstring{\(\rhn_{i}\to\nu_{j}h\)}{RH-Neutrino to LH-Neutrino and Higgs}}
The amplitude for \(\rhn_{i}(P) \to H(p_{h}) + \nu_j(p_{\nu})\) is given by:
\begin{align}
	\cM & = 2i \qty[G_{ij}y(p_{\nu})x(P) + G^{*}_{ij}x^{\dagger}(p_{\nu})y^{\dagger}(P)]
\end{align}
where \(G_{ij} = \qty(\bm{\cK}_{L}^{\dagger}\bm{\cK}_{R})_{ij}\). Squaring an summing
over spins, we find:
\begin{align}
	\frac{1}{2}\sum_{\mathrm{spins}}\qty|\cM|^2
	 & =
	4\qty[\qty(m_{\rhn}^2+m_{\nu_{j}}^2 - m_{h}^2) \qty|G_{ij}|^2 + 2m_{\rhn_{i}}m_{\nu_{j}}\Re(G_{ij}^2)]
\end{align}
The partial width is therefore:
\begin{align}
	\Gamma(\rhn_{i}\to \nu_{j}h)
	 & =
	\frac{\lambda^{1/2}(m^{2}_{\rhn_{i}},m_{\nu_{j}}^2,m_{h}^{2})}{16\pi v^{2}m^{3}_{\rhn^{2}_{i}}}
	\bigg{[}
	\qty(m_{\rhn_{i}}^4+m_{\nu_{j}}^4 - m_{h}^2\qty(m_{\rhn_{i}}^2+m_{\nu_{j}}^2) + 6m_{\rhn_{i}}^2m_{\nu_{j}}^2) \qty|G_{ij}|^2 \\
	 & \quad\quad + 2m_{\nu_{j}}m_{\rhn_{i}}\qty(2m_{\rhn_{i}}^2 + 2m_{\nu_{j}}^2 - m_{h}^2)\Re(G_{ij}^2)
	\bigg{]}\notag                                                                                                               \\
	 & \quad\times \theta(m_{\rhn_{i}}-m_{\nu_{j}}-m_{h})\notag
\end{align}

\subsubsection{\texorpdfstring{\(\rhn_{i}\to\nu_{j}Z\)}{RH-Neutrino to LH-Neutrino and Z-Boson}}
The amplitude for \(\rhn_{i}(P) \to Z(p_{Z}) + \nu_j(p_{\nu})\) is given by:
\begin{align}
    \cM & = -iG_{ij} \frac{e}{c_{W}s_{W}}\qty[x^{\dagger}(p_{\nu})\bar{\sigma}_{\mu}x(P)
        - y^{\dagger}(P)\bar{\sigma}_{\mu}y(p_{\nu})]\epsilon^{*}_{\mu}
\end{align}
where \(G_{ij} = \qty(\OmegaVVb^{\dagger}\OmegaVNb)_{ij}\). Squaring and summing
over spins, we find:
\begin{align}
    \frac{1}{2}\sum_{\mathrm{spins}}\qty|\cM|^2
     & =
    \frac{e^{2}\qty|G_{ij}|^2}{s^{2}_{W}M_{W}^{2}}
    \qty(\qty(m_{\rhn_{i}}+m_{\nu_{i}})^{2}-M_{Z}^{2})
    \qty(\qty(m_{\rhn_{i}}-m_{\nu_{i}})^{2}+2M_{Z}^{2})
\end{align}
The partial width is therefore:
% prefactor \lambda^{1/2}(m^{2}_{\rhn_{i}},m_{1}^2,m_{2}^{2}) / (16\pi m^{3}_{\rhn^{2}_{i}})
\begin{align}
    \Gamma(\rhn_{i}\to \nu_{j}Z)
     & =
    \frac{e^{2}\lambda^{1/2}(m^{2}_{\rhn_{i}},m_{\nu_{j}}^2,M_{Z}^{2})}{16\pi s^{2}_{W}M^{2}_{W}m^{3}_{\rhn^{2}_{i}}}
    \qty|\qty(\OmegaVVb^{\dagger}\OmegaVNb)_{ij}|^2
    \qty(\qty(m_{\rhn_{i}}+m_{\nu_{i}})^{2}-M_{Z}^{2})\notag          \\
     & \quad\times\qty(\qty(m_{\rhn_{i}}-m_{\nu_{i}})^{2}+2M_{Z}^{2})
    \theta(m_{\rhn_{i}}-m_{\nu_{j}}-M_{Z})
\end{align}

\subsubsection{\texorpdfstring{\(\rhn_{i}\to\ell_{j}W^{+}\)}{RH-Neutrino to Charged-Lepton and W-Boson}}
The amplitude for \(\rhn_{i}(P) \to W^{+}(p_{W}) + \ell_{j}(p_{\ell})\) is given by:
\begin{align}
    \cM & = -i\frac{e}{\sqrt{2}s_{W}}G_{ij} x^{\dagger}(p_{\ell})\bar{\sigma}_{\mu}x(P)
\end{align}
where \(G_{ij} = \qty(\OmegaVNb)_{ij}\). Squaring and summing
over spins, we find:
\begin{align}
    \frac{1}{2}\sum_{\mathrm{spins}}\qty|\cM|^2
     & =
    \frac{e^{2}\qty|\OmegaVNb^{ij}|^2}{4M_{W}^{2}}
    \qty(
    \qty(m_{\rhn_{i}}-m_{\ell_{j}})^{2}
    +\qty(m^{2}_{\rhn_{i}}+m^{2}_{\ell_{j}})M_{W}^{2}
    -2M_{W}^{4}
    )
\end{align}
The partial width is therefore:
% prefactor \lambda^{1/2}(m^{2}_{\rhn_{i}},m_{1}^2,m_{2}^{2}) / (16\pi m^{3}_{\rhn^{2}_{i}})
\begin{align}
    \Gamma(\rhn_{i}\to \ell_{j}W^{+})
     & =
    \frac{e^{2}\lambda^{1/2}(m^{2}_{\rhn_{i}},m_{\ell_{j}}^2,M_{W}^{2})}{64\pi M^{2}_{W}m^{3}_{\rhn^{2}_{i}}}
    \qty|\OmegaVNb^{ij}|^2
    \qty(
    \qty(m_{\rhn_{i}}-m_{\ell_{j}})^{2}
    +\qty(m^{2}_{\rhn_{i}}+m^{2}_{\ell_{j}})M_{W}^{2}
    -2M_{W}^{4}
    )\notag                                               \\
     & \quad\times\theta(m_{\rhn_{i}}-m_{\ell_{j}}-M_{W})
\end{align}
\subsubsection{\texorpdfstring{\(\rhn_{i}\to\nu_{j}\gamma\)}{RH-Neutrino to LH-Neutrino and Photon}}
In two component spinor notation, there are either 6 or 12 diagrams contributing to
\(\rhn_{i}\to\nu_{j}\gamma\) at one loop, depending on the gauge used. These are shown in
\FigRef{fig:n_to_nu_gamma_w} and \FigRef{fig:n_to_nu_gamma_ell}.

\begin{figure}[ht!]
    \centering
    \begin{subfigure}[b]{0.45\linewidth}
        \begin{tikzpicture}
            \begin{feynman}
                \vertex (i1)  {\(\rhn_{i}\)};
                \vertex[right=1cm of i1] (v1) ;
                \vertex[right=1cm of v1] (g1) ;
                \vertex[right=1cm of g1] (v2) ;
                \vertex[above=1cm of g1] (v3) ;
                \vertex[right=1cm of v2] (o1) {\(\nu_{j}\)};
                \vertex[above=1cm of v3] (g2) ;
                \vertex[right=1cm of g2] (o2) {\(\gamma\)};
                \diagram*{
                (i1) -- [fermion] (v1) -- [fermion,edge label=\(\ell_{k}\)](v2) -- [fermion](o1);
                (v1) -- [charged boson,quarter left,looseness=1.0,edge label=\(W^{+}\)] (v3) -- [charged boson,quarter left,looseness=1.0] (v2);
                (v3) -- [boson] (o2);
                };
            \end{feynman}
        \end{tikzpicture}
        \caption{}
    \end{subfigure}
    \begin{subfigure}[b]{0.45\linewidth}
        \begin{tikzpicture}
            \begin{feynman}
                \vertex (i1)  {\(\rhn_{i}\)};
                \vertex[right=1cm of i1] (v1) ;
                \vertex[right=1cm of v1] (g1) ;
                \vertex[right=1cm of g1] (v2) ;
                \vertex[above=1cm of g1] (v3) ;
                \vertex[right=1cm of v2] (o1) {\(\nu_{j}\)};
                \vertex[above=1cm of v3] (g2) ;
                \vertex[right=1cm of g2] (o2) {\(\gamma\)};
                \diagram*{
                (o1) -- [fermion] (v2) -- [fermion](v1) -- [fermion](i1);
                (v1) -- [anti charged boson,quarter left,looseness=1.0] (v3) -- [anti charged boson,quarter left,looseness=1.0] (v2);
                (v3) -- [boson] (o2);
                };
            \end{feynman}
        \end{tikzpicture}
        \caption{}
    \end{subfigure}
    \begin{subfigure}[b]{0.45\linewidth}
        \begin{tikzpicture}
            \begin{feynman}
                \vertex (i1)  {\(\rhn_{i}\)};
                \vertex[right=1cm of i1] (v1) ;
                \vertex[right=1cm of v1] (g1) ;
                \vertex[right=1cm of g1] (v2) ;
                \vertex[above=1cm of g1] (v3) ;
                \vertex[right=1cm of v2] (o1) {\(\nu_{j}\)};
                \vertex[above=1cm of v3] (g2) ;
                \vertex[right=1cm of g2] (o2) {\(\gamma\)};
                \diagram*{
                (i1) -- [fermion] (v1) -- [anti fermion,edge label=\(\ell_{k}\)](v2) -- [fermion](o1);
                (v1) -- [anti charged scalar,quarter left,looseness=1.0,edge label=\(G^{+}\)] (v3) -- [anti charged scalar,quarter left,looseness=1.0] (v2);
                (v3) -- [boson] (o2);
                };
            \end{feynman}
        \end{tikzpicture}
        \caption{}
    \end{subfigure}
    \begin{subfigure}[b]{0.45\linewidth}
        \begin{tikzpicture}
            \begin{feynman}
                \vertex (i1)  {\(\rhn_{i}\)};
                \vertex[right=1cm of i1] (v1) ;
                \vertex[right=1cm of v1] (g1) ;
                \vertex[right=1cm of g1] (v2) ;
                \vertex[above=1cm of g1] (v3) ;
                \vertex[right=1cm of v2] (o1) {\(\nu_{j}\)};
                \vertex[above=1cm of v3] (g2) ;
                \vertex[right=1cm of g2] (o2) {\(\gamma\)};
                \diagram*{
                (o1) -- [fermion] (v2) -- [anti fermion](v1) -- [fermion](i1);
                (v1) -- [charged scalar,quarter left,looseness=1.0] (v3) -- [charged scalar,quarter left,looseness=1.0] (v2);
                (v3) -- [boson] (o2);
                };
            \end{feynman}
        \end{tikzpicture}
        \caption{}
    \end{subfigure}
    \caption{Diagrams contributing to \(\rhn_{i}\to\nu_{j}\gamma\) with photon
        emission from \(W\)-boson.}
    \label{fig:n_to_nu_gamma_w}
\end{figure}

\begin{figure}[ht!]
    \centering
    \begin{subfigure}[b]{0.45\linewidth}
        \begin{tikzpicture}
            \begin{feynman}
                \vertex (i1)  {\(\rhn_{i}\)};
                \vertex[right=1cm of i1] (v1) ;
                \vertex[right=1cm of v1] (v2) ;
                \vertex[right=1cm of v2] (v3) ;
                \vertex[right=1cm of v3] (o1) {\(\nu_{j}\)};
                \vertex[below=1cm of v2] (g1) ;
                \vertex[right=1cm of g1] (o2) {\(\gamma\)};
                \diagram*{
                (i1) -- [fermion] (v1) -- [fermion,edge label'=\(\ell_{k}\)](v2) -- [fermion](v3) -- [fermion](o1);
                (v1) -- [charged boson,half left,looseness=1.5,edge label=\(W^{+}\)] (v3) ;
                (v2) -- [boson] (o2);
                };
            \end{feynman}
        \end{tikzpicture}
        \caption{}
    \end{subfigure}
    \begin{subfigure}[b]{0.45\linewidth}
        \begin{tikzpicture}
            \begin{feynman}
                \vertex (i1)  {\(\rhn_{i}\)};
                \vertex[right=1cm of i1] (v1) ;
                \vertex[right=1cm of v1] (v2) ;
                \vertex[right=1cm of v2] (v3) ;
                \vertex[right=1cm of v3] (o1) {\(\nu_{j}\)};
                \vertex[below=1cm of v2] (g1) ;
                \vertex[right=1cm of g1] (o2) {\(\gamma\)};
                \diagram*{
                (i1) -- [anti fermion] (v1) -- [anti fermion](v2) -- [anti fermion](v3) -- [anti fermion](o1);
                (v1) -- [anti charged boson,half left,looseness=1.5] (v3) ;
                (v2) -- [boson] (o2);
                };
            \end{feynman}
        \end{tikzpicture}
        \caption{}
    \end{subfigure}
    \begin{subfigure}[b]{0.45\linewidth}
        \begin{tikzpicture}
            \begin{feynman}
                \vertex (i1)  {\(\rhn_{i}\)};
                \vertex[right=1cm of i1] (v1) ;
                \vertex[right=1cm of v1] (v2) ;
                \vertex[right=1cm of v2] (v3) ;
                \vertex[right=1cm of v3] (o1) {\(\nu_{j}\)};
                \vertex[below=1cm of v2] (g3) ;
                \vertex[right=1cm of g3] (o2) {\(\gamma\)};
                \diagram*{
                (i1) -- [fermion] (v1) -- [majorana](v2) -- [anti majorana] (v3) -- [fermion](o1);
                (v1) -- [charged boson,half left,looseness=1.5] (v3) ;
                (v2) -- [boson] (o2);
                };
            \end{feynman}
        \end{tikzpicture}
        \caption{}
    \end{subfigure}
    \begin{subfigure}[b]{0.45\linewidth}
        \begin{tikzpicture}
            \begin{feynman}
                \vertex (i1)  {\(\rhn_{i}\)};
                \vertex[right=1cm of i1] (v1) ;
                \vertex[right=1cm of v1] (v2) ;
                \vertex[right=1cm of v2] (v3) ;
                \vertex[right=1cm of v3] (o1) {\(\nu_{j}\)};
                \vertex[below=1cm of v2] (g3) ;
                \vertex[right=1cm of g3] (o2) {\(\gamma\)};
                \diagram*{
                (i1) -- [anti fermion] (v1) -- [anti majorana](v2) -- [majorana] (v3) -- [anti fermion](o1);
                (v1) -- [anti charged boson,half left,looseness=1.5] (v3) ;
                (v2) -- [boson] (o2);
                };
            \end{feynman}
        \end{tikzpicture}
        \caption{}
    \end{subfigure}
    \begin{subfigure}[b]{0.45\linewidth}
        \begin{tikzpicture}
            \begin{feynman}
                \vertex (i1)  {\(\rhn_{i}\)};
                \vertex[right=1cm of i1] (v1) ;
                \vertex[right=1cm of v1] (v2) ;
                \vertex[right=1cm of v2] (v3) ;
                \vertex[right=1cm of v3] (o1) {\(\nu_{j}\)};
                \vertex[below=1cm of v2] (g1) ;
                \vertex[right=1cm of g1] (o2) {\(\gamma\)};
                \diagram*{
                (i1) -- [fermion] (v1) -- [anti fermion,edge label'=\(\ell_{k}\)](v2) -- [anti fermion](v3) -- [fermion](o1);
                (v1) -- [anti charged scalar,half left,looseness=1.5,edge label=\(G^{+}\)] (v3) ;
                (v2) -- [boson] (o2);
                };
            \end{feynman}
        \end{tikzpicture}
        \caption{}
    \end{subfigure}
    \begin{subfigure}[b]{0.45\linewidth}
        \begin{tikzpicture}
            \begin{feynman}
                \vertex (i1)  {\(\rhn_{i}\)};
                \vertex[right=1cm of i1] (v1) ;
                \vertex[right=1cm of v1] (v2) ;
                \vertex[right=1cm of v2] (v3) ;
                \vertex[right=1cm of v3] (o1) {\(\nu_{j}\)};
                \vertex[below=1cm of v2] (g1) ;
                \vertex[right=1cm of g1] (o2) {\(\gamma\)};
                \diagram*{
                (i1) -- [anti fermion] (v1) -- [fermion](v2) -- [fermion](v3) -- [anti fermion](o1);
                (v1) -- [charged scalar,half left,looseness=1.5] (v3) ;
                (v2) -- [boson] (o2);
                };
            \end{feynman}
        \end{tikzpicture}
        \caption{}
    \end{subfigure}
    \begin{subfigure}[b]{0.45\linewidth}
        \begin{tikzpicture}
            \begin{feynman}
                \vertex (i1)  {\(\rhn_{i}\)};
                \vertex[right=1cm of i1] (v1) ;
                \vertex[right=1cm of v1] (v2) ;
                \vertex[right=1cm of v2] (v3) ;
                \vertex[right=1cm of v3] (o1) {\(\nu_{j}\)};
                \vertex[below=1cm of v2] (g3) ;
                \vertex[right=1cm of g3] (o2) {\(\gamma\)};
                \diagram*{
                (i1) -- [fermion] (v1) -- [anti majorana](v2) -- [majorana] (v3) -- [fermion](o1);
                (v1) -- [anti charged scalar,half left,looseness=1.5] (v3) ;
                (v2) -- [boson] (o2);
                };
            \end{feynman}
        \end{tikzpicture}
        \caption{}
    \end{subfigure}
    \begin{subfigure}[b]{0.45\linewidth}
        \begin{tikzpicture}
            \begin{feynman}
                \vertex (i1)  {\(\rhn_{i}\)};
                \vertex[right=1cm of i1] (v1) ;
                \vertex[right=1cm of v1] (v2) ;
                \vertex[right=1cm of v2] (v3) ;
                \vertex[right=1cm of v3] (o1) {\(\nu_{j}\)};
                \vertex[below=1cm of v2] (g3) ;
                \vertex[right=1cm of g3] (o2) {\(\gamma\)};
                \diagram*{
                (i1) -- [anti fermion] (v1) -- [majorana](v2) -- [anti majorana] (v3) -- [anti fermion](o1);
                (v1) -- [charged scalar,half left,looseness=1.5] (v3) ;
                (v2) -- [boson] (o2);
                };
            \end{feynman}
        \end{tikzpicture}
        \caption{}
    \end{subfigure}
    \caption{Diagrams contributing to \(\rhn_{i}\to\nu_{j}\gamma\) with photon
        emission from charged lepton. Note diagrams use two-component spinors
        with (c), (d), (g) and (f) representing charged lepton mass insertions.}
    \label{fig:n_to_nu_gamma_ell}
\end{figure}

We will denote the \(W^{+}W^{-}\gamma\) vertex as \(V^{\alpha\beta\mu}(p^{+}_{\alpha},p^{-}_{\beta},p^{\gamma}_{\mu})\),
given by:
\begin{align}
	V_{WW\gamma}^{\alpha\beta\mu}(p^{+}_{\alpha},p^{-}_{\beta},p^{\gamma}_{\mu}) =
	ie\qty[
		g^{\alpha\beta}\qty(p^{-}-p^{+})_{\mu} +
		g^{\alpha\mu}\qty(p^{+}-p^{\gamma})_{\beta} +
		g^{\beta\mu}\qty(p^{\gamma}-p^{-})_{\alpha}
	]
\end{align}
We denote the \(G^{+}G^{-}\gamma\) vertex as \(V^{\mu}(p^{+},p^{-})\), given by:
\begin{align}
	V_{GG\gamma}^{\mu}(p^{+},p^{-}) = ie\qty(p^{+} - p^{-})_{\mu}
\end{align}
Note that \(V_{WW\gamma}^{\alpha\beta\mu}(p^{+}_{\alpha},p^{-}_{\beta},p^{\gamma}_{\mu}) = -V_{WW\gamma}^{\beta\alpha\mu}(p^{-}_{\alpha},p^{+}_{\beta},p^{\gamma}_{\mu})\)
and \(V_{GG\gamma}^{\mu}(p^{+},p^{-}) = - V_{GG\gamma}^{\mu}(p^{-},p^{+})\).
We use \(\Delta\) for a propagator. For example:
\begin{align}
	\Delta^{\mu\nu}_{W}(p) & = \frac{i}{p^2-M_{W}^{2}+i\epsilon}\qty(-g^{\mu\nu} + (1-\xi)\frac{p^{\mu}p^{\nu}}{p^{2}-\xi M_{W}^{2}}) \\
	\Delta^{G}(p)          & = \frac{i}{p^2-\xi M_{W}^{2}+i\epsilon}
\end{align}
In addition, we denote the neutrino interactions as:
\begin{align}
	V^{\mu}_{W\nu_{i}\ell_{j}}  & \equiv A = \frac{e}{\sqrt{2}\sw}\qty(\bm{\cK}_{L})^{ij}\bar{\sigma}_{\mu}     \\
	V^{\mu}_{W\rhn_{i}\ell_{j}} & \equiv B = \frac{e}{\sqrt{2}\sw}\qty(\bm{\cK}_{R})^{ij}\bar{\sigma}_{\mu}     \\
	V_{G\nu_{i}\ell_{j}}        & \equiv \tilde{A} =  \frac{e}{\sqrt{2}\sw}\qty(\hat{\bm{m}}_{D}\OmegaVVb)^{ij} \\
	V_{G\rhn_{i}\ell_{j}}       & \equiv \tilde{B} = \frac{e}{\sqrt{2}\sw}\qty(\hat{\bm{m}}_{D}\OmegaVNb)^{ij}
\end{align}

% ============================================================================
% ---- W-Emission Diagrams ---------------------------------------------------
% ============================================================================

The amplitude of the diagrams with \(W\)-bosons in \FigRef{fig:n_to_nu_gamma_w} are given by
\begin{align}
	i\cA^{(a)}_{1}
	 & =
	-i\qty(A^{*}B)
	\int\frac{\dd[4]{\ell}}{(2\pi)^{4}}
	\frac{x_{\nu}^{\dagger}(q)\bar{\sigma}_{\mu}\qty(\ell\cdot\sigma)\bar{\sigma}_{\nu}x_{\rhn}(p)}{\ell^{2}-m_{\ell_{k}}^{2}} \\
	 & \quad \times
	\Delta^{\nu\rho}_{W}(p-\ell)
	\Delta^{\lambda\mu}_{W}(\ell-q)
	V^{\rho\lambda\alpha}_{WW\gamma}(p-\ell,\ell-q,-k)
	\epsilon^{*}_{\alpha}(k)
	\notag                                                                                                                     \\
	%--------------------------
	i\cA^{(b)}_{1}
	 & =
	i\qty(AB^{*})
	\int\frac{\dd[4]{\ell}}{(2\pi)^{4}}
	\frac{y_{\nu}(q)\sigma_{\mu}\qty(\ell\cdot\bar{\sigma})\sigma_{\nu}y^{\dagger}_{\rhn}(p) }{\ell^{2}-m_{\ell_{k}}^{2}}      \\
	 & \quad \times
	\Delta^{\nu\rho}_{W}(p-\ell)
	\Delta^{\lambda\mu}_{W}(\ell-q)
	V^{\rho\lambda\alpha}_{WW\gamma}(p-\ell,\ell-q,-k)
	\epsilon^{*}_{\alpha}(k)
	\notag
\end{align}

% ============================================================================
% ---- G-Emission Diagrams ---------------------------------------------------
% ============================================================================

The amplitude of the diagrams with Goldstones in \FigRef{fig:n_to_nu_gamma_w} are given by
\begin{align}
	i\cA^{(c)}_{1}
	 & =
	-i\qty(\tilde{A}\tilde{B}^{*})
	\int\frac{\dd[4]{\ell}}{(2\pi)^{4}}
	\frac{x_{\nu}^{\dagger}(q)\qty[\ell\cdot\bar{\sigma}]x_{\rhn}(p)}{\ell^{2}-m_{\ell_{k}}^{2}}
	\\
	 & \quad \times
	\Delta^{G}(p-\ell)
	\Delta^{G}(\ell-q)
	V^{\alpha}_{GG\gamma}(p-\ell,\ell-q)
	\epsilon^{*}_{\alpha}(k)
	\notag          \\
	%--------------------------
	i\cA^{(d)}_{1}
	 & =
	i\qty(\tilde{A}^{*}\tilde{B})
	\int\frac{\dd[4]{\ell}}{(2\pi)^{4}}
	\frac{y_{\nu}(q)\qty[\ell\cdot\sigma]y^{\dagger}_{\rhn}(p)}{\ell^{2}-m_{\ell_{k}}^{2}}
	\\
	 & \quad \times
	\Delta^{G}(p-\ell)
	\Delta^{G}(\ell-q)
	V^{\alpha}_{GG\gamma}(p-\ell,\ell-q)
	\epsilon^{*}_{\alpha}(k)
	\notag
\end{align}

% ============================================================================
% ---- L-Emission Diagrams with W --------------------------------------------
% ============================================================================

The amplitudes for the diagrams with \(W\)-bosons in \FigRef{fig:n_to_nu_gamma_ell} are given by
\begin{align}
	i\cA^{(a)}_{2}
	 & =
	-ieA^{*}B
	\int\frac{\dd[4]{\ell}}{(2\pi)^{4}}
	\frac{
	x_{\nu}^{\dagger}(q)
	\bar{\sigma}_{\mu}
	\qty[\qty(q-\ell)\cdot\sigma]
	\bar{\sigma}_{\alpha}
	\qty[\qty(p-\ell)\cdot\sigma]
	\bar{\sigma}_{\nu}
	x_{\rhn}(p)
	}{
	\qty[\qty(p-\ell)^{2}-m_{\ell_{k}}^{2}]\qty[\qty(q-\ell)^{2}-m_{\ell_{k}}^{2}]
	}
	\Delta^{\mu\nu}_{W}(\ell)
	\epsilon^{*}_{\alpha}(k)
	\\
	%--------------------------
	i\cA^{(b)}_{2}
	 & =
	ieAB^{*}
	\int\frac{\dd[4]{\ell}}{(2\pi)^{4}}
	\frac{
	y_{\nu}(q)
	\sigma_{\mu}
	\qty[\qty(q-\ell)\cdot\bar{\sigma}]
	\sigma_{\alpha}
	\qty[\qty(p-\ell)\cdot\bar{\sigma}]
	\sigma_{\nu}
	y_{\rhn}^{\dagger}(p)
	}{
	\qty[\qty(q-\ell)^{2}-m_{\ell_{k}}^{2}]\qty[\qty(p-\ell)^{2}-m_{\ell_{k}}^{2}]
	}
	\Delta^{\mu\nu}_{W}(\ell)
	\epsilon^{*}_{\alpha}(k)
	\\
	i\cA^{(c)}_{2}
	 & =
	-ieA^{*}B m^{2}_{\ell_{k}}
	\int\frac{\dd[4]{\ell}}{(2\pi)^{4}}
	\frac{
	x_{\nu}^{\dagger}(q)
	\bar{\sigma}_{\mu}\sigma_{\alpha}\bar{\sigma}_{\nu}
	x_{\rhn}(p)
	}{
	\qty[\qty(q-\ell)^{2}-m_{\ell_{k}}^{2}]\qty[\qty(p-\ell)^{2}-m_{\ell_{k}}^{2}]
	}
	\Delta^{\mu\nu}_{W}(\ell)
	\epsilon^{*}_{\alpha}(k)
	\\
	i\cA^{(d)}_{2}
	 & =
	ieAB^{*}m^{2}_{\ell_{k}}
	\int\frac{\dd[4]{\ell}}{(2\pi)^{4}}
	\frac{
	y_{\nu}(q)
	\sigma_{\mu}
	\bar{\sigma}_{\alpha}
	\sigma_{\nu}
	y_{\rhn}^{\dagger}(p)
	}{
	\qty[\qty(q-\ell)^{2}-m_{\ell_{k}}^{2}]\qty[\qty(p-\ell)^{2}-m_{\ell_{k}}^{2}]
	}
	\Delta^{\mu\nu}_{W}(\ell)
	\epsilon^{*}_{\alpha}(k)
\end{align}

% ============================================================================
% ---- L-Emission Diagrams with G --------------------------------------------
% ============================================================================

The amplitudes for the diagrams with Goldstones in \FigRef{fig:n_to_nu_gamma_ell} are given by
\begin{align}
	i\cA^{(e)}_{2}
	 & =
	-ie\tilde{A}\tilde{B}^{*}
	\int\frac{\dd[4]{\ell}}{(2\pi)^{4}}
	\frac{
	x_{\nu}^{\dagger}(q)
	\qty[\qty(q-\ell)\cdot\bar{\sigma}]\sigma_{\alpha}\qty[\qty(p-\ell)\cdot\bar{\sigma}]
	x_{\rhn}(p)
	}{
	\qty[\qty(q-\ell)^{2}-m_{\ell_{k}}^{2}]\qty[\qty(p-\ell)^{2}-m_{\ell_{k}}^{2}]
	}
	\Delta^{G}(\ell)
	\epsilon^{*}_{\alpha}(k)
	\\
	%--------------------------
	i\cA^{(f)}_{2}
	 & =
	-ie\tilde{A}^{*}\tilde{B}
	\int\frac{\dd[4]{\ell}}{(2\pi)^{4}}
	\frac{
	y_{\nu}(q)
	\qty[\qty(q-\ell)\cdot\sigma]\bar{\sigma}_{\alpha}\qty[\qty(p-\ell)\cdot\sigma]
	y_{\rhn}^{\dagger}(p)
	}{
	\qty[\qty(q-\ell)^{2}-m_{\ell_{k}}^{2}]\qty[\qty(p-\ell)^{2}-m_{\ell_{k}}^{2}]
	}
	\Delta^{G}(\ell)
	\epsilon^{*}_{\alpha}(k)
	\\
	i\cA^{(g)}_{2}
	 & =
	ie\tilde{A}\tilde{B}^{*}m^{2}_{\ell_{k}}
	\int\frac{\dd[4]{\ell}}{(2\pi)^{4}}
	\frac{
	x_{\nu}^{\dagger}(q)\bar{\sigma}_{\alpha}x_{\rhn}(p)
	}{
	\qty[\qty(q-\ell)^{2}-m_{\ell_{k}}^{2}]\qty[\qty(p-\ell)^{2}-m_{\ell_{k}}^{2}]
	}
	\Delta^{G}(\ell)
	\epsilon^{*}_{\alpha}(k)
	\\
	i\cA^{(h)}_{2}
	 & =
	-ie\tilde{A}^{*}\tilde{B}m^{2}_{\ell_{k}}
	\int\frac{\dd[4]{\ell}}{(2\pi)^{4}}
	\frac{
	y_{\nu}(q)\sigma_{\alpha}y_{\rhn}^{\dagger}(p)
	}{
	\qty[\qty(q-\ell)^{2}-m_{\ell_{k}}^{2}]\qty[\qty(p-\ell)^{2}-m_{\ell_{k}}^{2}]
	}
	\Delta^{G}(\ell)
	\epsilon^{*}_{\alpha}(k)
\end{align}

\subsubsection{\texorpdfstring{\(\rhn_{i}\to\nu_{j}\pi^{0},\nu_{j}\eta\)}{RH-Neutrino to LH-Neutrino and Neutral Pion}}

The relavent interactions for \(\rhn_{i}\to\nu_{j}\pi^{0}\) stem from
\begin{align}
    \cL_{4F} & = -\frac{4\gf\fpi}{2\cw^{2}\sqrt{2}}\qty(\partial_{\mu}\piz)
    \qty(\qty(\OmegaVVb^{\dagger}\OmegaVNb)^{ij}
    \nu_{i}^{\dagger}
    \bar{\sigma}_{\mu}
    \rhn_{j}
    +\qty(\OmegaVNb^{\dagger}\OmegaVVb)^{ij}\rhn_{i}^{\dagger}
    \bar{\sigma}_{\mu}
    \nu_{j}
    )
\end{align}
Thus, the amplitude is given by:
\begin{align}
    i\cM\qty(\rhn_{i}\to\nu_{j}\pi^{0})
    =
    -i\frac{\sqrt{2}\gf\fpi}{\cw^{2}}\qty(i p^{\mu}_{\piz})
    \qty[
    gx^{\dagger}_{\nu}\bar{\sigma}_{\mu}x_{\rhn}
    -
    g^{*}y^{\dagger}_{\rhn}\bar{\sigma}_{\mu}y_{\nu}
    ]
\end{align}
where \(g\equiv \qty(\OmegaVVb^{\dagger}\OmegaVNb)^{ij}\).
Squaring and summing over spins yields:
\begin{align}
    \frac{1}{2}\sum_{\mathrm{spins}}\qty|\cM\qty(\rhn_{i}\to\nu_{j}\pi^{0})|^{2}
     & =
    \frac{2\gf^{2}\fpi^{2}}{\cw^{4}}
    \bigg{[}
    |g|^{2}\qty(\qty(m_{\rhn_{i}}^{2}-m_{\nu_{j}}^{2})^{2}
    - m_{\piz}^{2}\qty(m_{\rhn_{i}}^{2}+m_{\nu_{j}}^{2})) \\
     & \qquad\qquad\qquad
    -4\Re(g^2)m_{\rhn_{i}}m_{\nu_{j}}m_{\piz}^{2}
    \bigg{]}\notag
\end{align}
and thus, the partial width is:
\begin{align}
    \Gamma\qty(\rhn_{i}\to\nu_{j}\pi^{0})
    =
    \frac{\gf^{2}\fpi^{2}m^{3}_{\rhn_{i}}}{8\pi \cw^{4}}
    \lambda^{1/2}(1,\beta_{\nu_{j}}^2,\beta_{\pi}^{2})
     &
    \bigg{[}
    |g|^{2}\qty(\qty(1-\beta_{\nu_{j}}^{2})^{2}
    - \beta_{\piz}^{2}\qty(1+\beta_{\nu_{j}}^{2})) \\
     & \quad
    -4\Re(g^2)\beta_{\nu_{j}}\beta_{\piz}^{2}
    \bigg{]}\notag
\end{align}
The result for \(\rhn_{i}\to\nu_{j}\eta\) is identical but has an extra factor of
\(1/3\)
\begin{align}
    \Gamma\qty(\rhn_{i}\to\nu_{j}\eta)
    =
    \frac{\gf^{2}\fpi^{2}m^{3}_{\rhn_{i}}}{24\pi \cw^{4}}
    \lambda^{1/2}(1,\beta_{\nu_{j}}^2,\beta_{\eta}^{2})
     &
    \bigg{[}
    |g|^{2}\qty(\qty(1-\beta_{\nu_{j}}^{2})^{2}
    - \beta_{\eta}^{2}\qty(1+\beta_{\nu_{j}}^{2})) \\
     & \quad
    -4\Re(g^2)\beta_{\nu_{j}}\beta_{\eta}^{2}
    \bigg{]}\notag
\end{align}

\subsubsection{\texorpdfstring{\(\rhn_{i}\to\ell_{j}\pip,\ell_{j}\kp\)}{RH-Neutrino to Charged Lepton and Charged Pion}}

The relavent interactions for \(\rhn_{i}\to\ell_{j}\pip\) stem from
\begin{align}
    \cL_{4F} & = -2\gf\fpi\vud\qty(\partial_{\mu}\pim)
    \qty(\OmegaVNb)^{ji}
    \ell_{j}^{\dagger}
    \bar{\sigma}_{\mu}
    \rhn_{i}
\end{align}
Thus, the amplitude is given by:
\begin{align}
    i\cM\qty(\rhn_{i}\to\ell_{j}\pip)
    =
    -2g\gf\fpi\vud\qty(ip_{\pip})
    x^{\dagger}_{\ell}\bar{\sigma}_{\mu}x_{\rhn}
\end{align}
where \(g\equiv \qty(\OmegaVNb)^{ji}\).
Squaring and summing over spins yields:
\begin{align}
    \frac{1}{2}\sum_{\mathrm{spins}}\qty|\cM\qty(\rhn_{i}\to\ell_{j}\pip)|^{2}
     & =
    2\qty|g|^{2}\gf^{2}\fpi^{2}\qty|\vud|^{2}
    \qty[\qty(m_{\rhn_{i}}^{2}-m_{\ell_{j}}^{2})^{2}
        - m_{\pip}^{2}\qty(m_{\rhn_{i}}^{2}+m_{\ell_{j}}^{2})]
\end{align}
and thus, the partial width is:
\begin{align}
    \Gamma\qty(\rhn_{i}\to\ell_{j}\pip)
    =
    \frac{\qty|g|^{2}\gf^{2}\fpi^{2}\qty|\vud|^{2}m^{3}_{\rhn_{i}}}{8\pi}
    \lambda^{1/2}(1,\beta_{\ell}^2,\beta_{\pip}^{2})
    \qty[\qty(1-\beta_{\ell_{j}}^{2})^{2}
        - \beta_{\pip}^{2}\qty(1+\beta_{\ell_{j}}^{2})]
\end{align}
The result for \(\rhn_{i}\to\ell_{j}K^{+}\) is obtained from the above with
the replacements \(V_{ud}\to V_{us}\) and \(\beta_{\pip}\to\beta_{\kp}\)
\begin{align}
    \Gamma\qty(\rhn_{i}\to\ell_{j}\kp)
    =
    \frac{\qty|g|^{2}\gf^{2}\fpi^{2}\qty|\vus|^{2}m^{3}_{\rhn_{i}}}{8\pi}
    \lambda^{1/2}(1,\beta_{\ell}^2,\beta_{\kp}^{2})
    \qty[\qty(1-\beta_{\ell_{j}}^{2})^{2}
        - \beta_{\kp}^{2}\qty(1+\beta_{\ell_{j}}^{2})]
\end{align}

\subsection{Three-Body Partial Widths}
Here we compute the partial widths of the general RH neutrino model into three-body
final states.

\subsubsection{\texorpdfstring{\(\rhn_{i}\to\nu_{j}q\bar{q}\)}{RH-Neutrino to LH-Neutrino and Quarks}}
The amplitude for \(\rhn_{i}(P) \to \nu_{j}(p_{\nu}) + q(p_{q}) + \bar{q}(p_{\bar{q}})\), where
\(q \in \qty{u,c,t,d,s,b}\) is a SM quark, contains a Z and a Higgs exchanged diagram. The diagrams are given by:
\begin{align}
    i\cM
     & =
    \qty[iG_{ij}y_{\nu}x_{\rhn} + iG^{*}_{ij}x^{\dagger}_{\nu}y^{\dagger}_{\rhn}]
    \qty(i\Delta_{h})
    \qty(-i\frac{m_{q}}{v})
    \qty[x^{\dagger}_{q}x^{\dagger}_{\bar{q}} + y_{u}y_{\bar{q}}] \\
     & \quad +
    \qty(i\tilde{G}_{ij})
    \qty[x^{\dagger}_{\nu}\bar{\sigma}^{\mu}x_{\rhn} - y^{\dagger}_{\rhn}\bar{\sigma}^{\mu}y_{\nu}]
    \qty(i\Delta^{\mu\nu}_{Z})
    \qty[ig^{q}_{L}x^{\dagger}_{q}\bar{\sigma}^{\mu}y_{\bar{q}} -ig^{q}_{R}x^{\dagger}_{\bar{q}}\bar{\sigma}^{\mu}y_{q}]
\end{align}
where \(G_{ij} = \qty(\OmegaNNb^{T}\hat{\bm{m}}\OmegaNVb)_{ij}\),
\(\tilde{G}_{ij} = (e/c_{W}s_{W})\qty(\OmegaVVb^{\dagger}\OmegaVN)_{ij}\) and the left and right handed
quark couplings to the Z are:
\begin{align}
    g^{q}_{L} & = \frac{e}{c_{W}s_{W}}\qty(T^{3}_{q} - s^{2}_{W}Q_{q}), &
    g^{q}_{R} & = \frac{e s_{W}}{c_{W}}Q_{q}
\end{align}
with \(T^{3}_{u} = 1/2, Q_{u}=2/3\) for up-type quarks and
\(T^{3}_{d} = -1/2, Q_{d}=-1/3\) for down-type quarks.
\(\Delta_{h}\) and \(\Delta^{\mu\nu}_{Z}\) are propagators for the Higgs and
Z-boson (in the unitary gauge) given by:
\begin{align}
    \Delta_{h}(p)
                                                   & =
    \frac{1}{p^2 - M^{2}_{h} + i M_{h}\Gamma_{h}}, &
    \Delta^{\mu\nu}_{Z}(p)
                                                   & =
    \frac{1}{p^2 - M^{2}_{Z} + i M_{Z}\Gamma_{Z}}
    \qty(-g^{\mu\nu} + \frac{p^{\mu}p^{\nu}}{M^{2}_{Z}})
\end{align}
Squaring and summing over spins, we find:
\begin{align}
    \frac{1}{2}\sum_{\mathrm{spins}}\qty|\cM|^2
     & =
    \frac{1}{2}\qty(
    N Q \qty|\Delta_{h}|^{2}
    + \qty[N_{\mu}Q_{\nu}\Delta^{\mu\nu}_{Z}\qty(\Delta_{H})^{*} + \mathrm{c.c}]
    + N_{\mu\alpha} Q_{\nu\beta}\Delta_{Z}^{\mu\nu}\qty(\Delta_{Z}^{\alpha\beta})^{*}
    )
\end{align}
where
\begin{align}
    N
     & =
    2\qty(
    \Re(G^{2}_{ij})m_{\nu_{j}}m_{\rhn_{i}}+4\qty|G_{ij}|^{2}\qty(P\cdot p_{\nu})
    )
    \\
    Q
     & = -\frac{4m^{2}_{u_{k}}}{v^{2}}\qty(m^{2}_{u_{k}} - p_{u}p_{\bar{u}})
    \\
    N^{\mu}
     & =
    \frac{2e}{c_{W}s_{W}}\qty(
    \mathrm{Im}\qty(G_{ij}\qty(\tilde{G}_{ij})^{*})m_{\nu_{j}}P^{\mu}
    - m_{\rhn_{i}}\Im(G_{ij}\tilde{G}_{ij})p^{\mu}_{\nu}
    )
    \\
    Q^{\mu}
     & =
    \frac{2m_{u_{k}}^{2}}{v}\qty(g_{L,q}-g_{R,q})(p^{\mu}_{u}-p^{\mu}_{\bar{u}})
    \\
    N^{\mu\alpha}
     & =
    -2\qty(
    2\Re(\tilde{G}_{ij})m_{\nu_{j}}m_{\rhn_{i}}g^{\mu\alpha}
    -2\qty|\tilde{G}_{ij}|^{2}\qty(
    P^{\alpha}p^{\mu}_{\nu} +
    P^{\mu}p^{\alpha}_{\nu}-\qty(P\cdot p_{\nu})g^{\mu\alpha}
    )
    )                                                                        \\
    Q^{\nu\beta}
     & =
    2\qty(g^{2}_{L,q} + g^{2}_{R,q})
    \qty(
    p^{\nu}_{u}p^{\beta}_{\bar{u}} +
    p^{\beta}_{u}p^{\nu}_{\bar{u}}
    )
    -2\qty(\qty(g^{2}_{L,q} + g^{2}_{R,q})\qty(p_{u}\cdot p_{\bar{u}})
    -2g_{L,q}g_{R,q}m^{2}_{u_{k}}
    )
\end{align}
