# Supplementary material for: Sterile Neutrinos from Dark Matter: A $\nu$ Nightmare?
Source: arXiv:2211.05996 source file (2022-11-11)
Supplement: Supplementary file 5 [file feynman_rules.tex]

% ============================================================================
% ---- W-Z Diagrams ----------------------------------------------------------
% ============================================================================

% ============================================================================
% ---- Z Diagrams ------------------------------------------------------------
% ============================================================================

% ============================================================================
% ---- Goldstone Diagrams with LH charged lepton -----------------------------
% ============================================================================

% ============================================================================
% ---- Goldstone Diagrams with RH charged lepton -----------------------------
% ============================================================================
