# Supplementary material for: Sterile Neutrinos from Dark Matter: A $\nu$ Nightmare?
Source: arXiv:2211.05996 source file (2022-11-11)
Supplement: Supplementary file 6 [file interactions.tex]

First, we consider the kinetic term for the lepton doublet:
\begin{align}
	L^{\dagger}_{a,i}\bar{\sigma}_{\mu}D^{\mu}L_{a,i} =
	\frac{e}{\sqrt{2}s_{W}}W^{-}_{\mu}\ell_{i}^{\dagger}\bar{\sigma}^{\mu}\hat{\nu}_{i}
	+\frac{e}{\sqrt{2}s_{W}}W^{+}_{\mu}\hat{\nu}_{i}^{\dagger}\bar{\sigma}^{\mu}\ell_{i}
	-\frac{e}{2c_{W}s_{W}}Z_{\mu}\hat{\nu}_{i}^{\dagger}\bar{\sigma}^{\mu}\hat{\nu}_{i} + \cdots
\end{align}
Rotating the neutrinos, we find
\begin{align}
	L^{\dagger}_{a,i}\bar{\sigma}_{\mu}D^{\mu}L_{a,i}
	 & = \cdots
	%----------
	+\frac{e}{\sqrt{2}s_{W}}W^{-}_{\mu}\ell_{i}^{\dagger}\bar{\sigma}^{\mu}
	\qty(\OmegaVVb)^{ij}\nu_{j}
	+\frac{e}{\sqrt{2}s_{W}}W^{-}_{\mu}\ell_{i}^{\dagger}\bar{\sigma}^{\mu}
	\qty(\OmegaVNb)^{ij}\rhn_{j}\notag                                                                                    \\
	%----------
	 & \quad
	+\frac{e}{\sqrt{2}s_{W}}W^{+}_{\mu}\nu_{i}^{\dagger}
	\qty(\OmegaVVb^{\dagger})^{ij}\bar{\sigma}^{\mu}\ell_{j}
	+\frac{e}{\sqrt{2}s_{W}}W^{+}_{\mu}\rhn_{i}^{\dagger}
	\qty(\OmegaVNb^{\dagger})^{ij}\bar{\sigma}^{\mu}\ell_{j}\notag                                                        \\
	%----------
	 & \quad
	+\frac{e}{2c_{W}s_{W}}Z_{\mu}\nu_{i}^{\dagger}\qty(\OmegaVVb^{\dagger}\OmegaVVb)^{in}\bar{\sigma}^{\mu}\nu_{j}
	+\frac{e}{2c_{W}s_{W}}Z_{\mu}\nu_{i}^{\dagger}\qty(\OmegaVVb^{\dagger}\OmegaVNb)^{in}\bar{\sigma}^{\mu}\rhn_{j}\notag \\
	%----------
	 & \quad
	+\frac{e}{2c_{W}s_{W}}Z_{\mu}\rhn_{n}^{\dagger}\qty(\OmegaVNb^{\dagger}\OmegaVVb)^{ij}\bar{\sigma}^{\mu}\nu_{j}
	+\frac{e}{2c_{W}s_{W}}Z_{\mu}\rhn_{n}^{\dagger}\qty(\OmegaVNb^{\dagger}\OmegaVNb)^{ij}\bar{\sigma}^{\mu}\rhn_{j}\notag
	%----------
\end{align}
Written in this way, we can interpret parts of mixing matrix. From the first two terms, we identify
\(\OmegaVVb\) as the PMNS matrix and
\(\OmegaVNb\) and its right-handed partner. We will now rename
\(\OmegaVVb\) as \(\bm{\cK}_{L}\) and
\(\OmegaVNb\) as \(\bm{\cK}_{R}\). Then, the above can be
written as
\begin{align}
	% \qty(\OmegaVVb)^{ij}\nu_{j} + \qty(\OmegaVNb)^{ij}\rhn_{j}
	% \qty(\OmegaNVb)^{ij}\nu_{j} + \qty(\OmegaNNb)^{ij}\rhn_{j}
	L^{\dagger}_{a,i}\bar{\sigma}_{\mu}D^{\mu}L_{a,i}
	 & = \cdots
	%----------
	+\frac{e}{\sqrt{2}s_{W}}W^{-}_{\mu}\ell_{i}^{\dagger}\bar{\sigma}^{\mu}\qty(\bm{\cK}_{L})^{ij}\nu_{j}
	+\frac{e}{\sqrt{2}s_{W}}W^{-}_{\mu}\ell_{i}^{\dagger}\bar{\sigma}^{\mu}\qty(\bm{\cK}_{R})^{ij}\rhn_{j}\notag                \\
	%----------
	 & \quad
	+\frac{e}{\sqrt{2}s_{W}}W^{+}_{\mu}\nu_{i}^{\dagger}\qty(\bm{\cK}_{L}^{\dagger})^{ij}\bar{\sigma}^{\mu}\ell_{j}
	+\frac{e}{\sqrt{2}s_{W}}W^{+}_{\mu}\rhn_{i}^{\dagger}\qty(\bm{\cK}_{R}^{\dagger})^{ij}\bar{\sigma}^{\mu}\ell_{j}\notag      \\
	%----------
	 & \quad
	+\frac{e}{2c_{W}s_{W}}Z_{\mu}\nu_{i}^{\dagger}\qty(\bm{\cK}_{L}^{\dagger}\bm{\cK}_{L})^{ij}\bar{\sigma}^{\mu}\nu_{j}
	+\frac{e}{2c_{W}s_{W}}Z_{\mu}\nu_{i}^{\dagger}\qty(\bm{\cK}_{L}^{\dagger}\bm{\cK}_{R})^{ij}\bar{\sigma}^{\mu}\rhn_{j}\notag \\
	%----------
	 & \quad
	+\frac{e}{2c_{W}s_{W}}Z_{\mu}\rhn_{i}^{\dagger}\qty(\bm{\cK}_{R}^{\dagger}\bm{\cK}_{L})^{ij}\bar{\sigma}^{\mu}\nu_{j}
	+\frac{e}{2c_{W}s_{W}}Z_{\mu}\rhn_{i}^{\dagger}\qty(\bm{\cK}_{R}^{\dagger}\bm{\cK}_{R})^{ij}\bar{\sigma}^{\mu}\rhn_{j}\notag
	%----------
\end{align}
Expanding out the Yukawa term in Eqn.~(\ref{eqn:GeneralRHN}), we find:
\begin{align}
	\Phi_{a}\epsilon^{ab}\hat{L}_{b,i}\bm{Y}^{ij}_{\nu}\hat{\rhn}_{j}
	 & =
	\frac{2}{v}G^{+}\ell_{i}\qty(\hat{\bm{m}})^{ij}_{D}\hat{\rhn}_j +
	\frac{1}{v}(h + iG^{0})\hat{\nu}_i\hat{\bm{m}}^{ij}_{D}\hat{\rhn}_{j}
	+ \frac{1}{v}\hat{\nu}_i\hat{\bm{m}}^{ij}_{D}\hat{\rhn}_{j} \\
	-\Phi_{a}^{\dagger}\hat{L}_{a,i}\bm{Y}^{ij}_{\ell}\hat{\bar{\ell}}_{j}
	 & =
	-\frac{\sqrt{2}}{v}G^{-}m_{\ell_{i}}\bar{\ell}_{i}\hat{\nu}_{i} +\cdots
\end{align}
Rotating the neutrinos, and using:
\begin{align}
	\hat{\bm{m}}_{D}\OmegaNVb & = \bm{\cK}_{L}^{*}\bm{m}_{\nu}, & %  \\
	\hat{\bm{m}}_{D}\OmegaNNb & = \bm{\cK}_{R}^{*}\bm{m}_{\rhn}   %                                                                                   \\
	%\OmegaNVb^{T}\hat{\bm{m}}\OmegaNVb & = \bm{m}_{\nu} - \bm{\cK}_{L}^{T}\bm{\cK}_{L}^{*}\bm{m}_{\nu} - \bm{m}_{\nu}\bm{\cK}_{L}^{\dagger}\bm{\cK}_{L}    \\
	%\OmegaNVb^{T}\hat{\bm{m}}\OmegaNNb & = -\bm{\cK}_{L}^{T}\bm{\cK}_{R}^{*}\bm{m}_{\rhn} - \bm{m}_{\nu}\bm{\cK}_{L}^{\dagger}\bm{\cK}_{R}                 \\
	%\OmegaNNb^{T}\hat{\bm{m}}\OmegaNNb & = \bm{m}_{\rhn} - \bm{\cK}_{R}^{T}\bm{\cK}_{R}^{*}\bm{m}_{\rhn} - \bm{m}_{\rhn}\bm{\cK}_{R}^{\dagger}\bm{\cK}_{R}
\end{align}
we find the following
\begin{align}
	\Phi_{a}\epsilon^{ab}\hat{L}_{b,i}\bm{Y}^{ij}_{\nu}\hat{\rhn}_{j} =
	%-----------------------------------------------------------
	 & \quad
	\frac{\sqrt{2}}{v}G^{+}\ell_{i}{\qty(\bm{\cK}_{L}^{*}\bm{m}_{\nu})}^{ij}\nu_{j}
	+ \frac{\sqrt{2}}{v}G^{+}\ell_{i}{\qty(\bm{\cK}_{R}^{*}\bm{m}_{\nu})}^{ij}\rhn_{j}
	\\
	%-----------------------------------------------------------
	 & \quad
	- \frac{h+iG^{0}}{v}\nu_i\qty(
	\bm{\cK}_{L}^{T}\bm{\cK}_{L}^{*}\bm{m}_{\nu}
	)^{ij}\nu_{j}
	- \frac{h+iG^{0}}{v}\rhn_i\qty(
	\bm{\cK}_{R}^{T}\bm{\cK}_{R}^{*}\bm{m}_{\rhn}
	)^{ij}\rhn_{j}
	\notag   \\
	%-----------------------------------------------------------
	 & \quad
	- \frac{h+iG^{0}}{v}\nu_i\qty(
	\bm{\cK}_{L}^{T}\bm{\cK}_{R}^{*}\bm{m}_{\rhn}
	)^{ij}\rhn_{j}
	- \frac{h+iG^{0}}{v}\rhn_i\qty(
	\bm{\cK}_{R}^{T}\bm{\cK}_{L}^{*}\bm{m}_{\nu}
	)^{ij}\nu_{j}
	\notag
\end{align}
The interactions with the right-handed charged leptons are:
\begin{align}
	-\Phi_{a}^{\dagger}\hat{L}_{a,i}\bm{Y}^{ij}_{\ell}\hat{\bar{\ell}}_{j}
	 & =
	-\frac{\sqrt{2}}{v}G^{-}\qty(\bm{m}_{\ell}\bm{\cK}_{L})^{ij}\bar{\ell}_{i}\nu_{j}
	-\frac{\sqrt{2}}{v}G^{-}\qty(\bm{m}_{\ell}\bm{\cK}_{R})^{ij}\bar{\ell}_{i}\rhn_{j}
\end{align}
