# Supplementary material for: Sterile Neutrinos from Dark Matter: A $\nu$ Nightmare?
Source: arXiv:2211.05996 source file (2022-11-11)
Supplement: Supplementary file 7 [file lagrangian.tex]

In this paper, we considered simplified cases where we assumed that the RHN of interest mixes with a single SM neutrino flavor, without considering the details of neutrino masses and mixings. In this appendix, we discuss such details for completeness.

Consider a theory with \(n\) right-handed neutrinos \(\hat{\rhn}_1, \dots, \hat{\rhn}_n\) that
interact with the standard model through a Yukawa interaction. The general
renormalizable Lagrangian for this theory is
\begin{align}\label{eqn:GeneralRHN}
	\mathcal{L}\supset
	\hat{\rhn}_i^{\dagger}\bar{\sigma}_{\mu}\partial^{\mu}\hat{\rhn}_i
	-\frac{1}{2}\qty(\hat{\bm{m}}^{ij}\hat{\rhn}_i\hat{\rhn}_j + \mathrm{c.c.})
	+ \qty(\Phi_{a}\epsilon^{ab}\hat{L}_{b,i}\bm{Y}^{ij}_{\nu}\hat{\rhn}_{j}
	- \Phi_{a}^{\dagger}\hat{L}_{a,i}\bm{Y}^{ij}_{\ell}\hat{\bar{\ell}}_{j} + \mathrm{c.c})
\end{align}
where \(\hat{\bm{m}}\) is an \(n\times n\) complex symmetric matrix, and
\(\bm{Y}_{\nu}\) is a \(3\times n\) complex matrix. Here \(\Phi\) is the Higgs doublet
\begin{align}
	\Phi = \frac{1}{\sqrt{2}}\mqty(\sqrt{2}G^{+} \\ v + h + iG^{0})
\end{align}
with \(v = 246 \ \mathrm{GeV}\) being the Higgs vacuum expectation value, \(h\)
the Higgs and \(G^{+},G^{0}\) the changed and neutral Goldstones. The lepton
doublet is parameterized as:
\begin{align}
	\hat{L}_{i} = \mqty(\hat{\nu}_i \\ \hat{\ell}_i)
\end{align}
with \(i\in\qty{1,2,3}\). \(\hat{\nu}_i\) are the left-handed neutrinos and
\(\ell_i\) are the gauge eigenstates of the charged leptons.
