# Supplementary material for: Sterile Neutrinos from Dark Matter: A $\nu$ Nightmare?
Source: arXiv:2211.05996 source file (2022-11-11)
Supplement: Supplementary file 8 [file mass_diag.tex]

Expanding out \ref{eqn:GeneralRHN}, the mass terms for the neutrinos are:
\begin{align}\label{eqn:RHNMass}
	\cL_{\nu,\mathrm{mass}}\supset
	-\frac{1}{2}\qty(\hat{\bm{m}}^{ij}\hat{\rhn}_i\hat{\rhn}_j + \mathrm{c.c.})
	- \frac{v}{\sqrt{2}}\qty(\hat{\nu}_{i}\bm{Y}^{ij}_{\nu}\hat{\rhn}_{j} + \mathrm{c.c})
\end{align}
Gathering the left- and right-handed neutrinos into a vector
\begin{align}
	\hat{\cN} = \mqty(\hat{\nu}_1 & \hat{\nu}_2 & \hat{\nu}_3 & \hat{\rhn}_1 & \cdots & \hat{\rhn}_n)^{T}
\end{align}
we can write the mass terms as:
\begin{align}\label{eqn:RHNMassMatrix}
	\cL_{\nu,\mathrm{mass}}
	                  & \supset
	-\frac{1}{2}\hat{\cN}_{i}\bm{M}^{ij}\hat{\cN}_j,
	                  &
	\hat{\bm{M}}      & = \mqty(
	\bm{0}_{3\times3} & \hat{\bm{m}}_{D} \\
	\hat{\bm{m}}_{D}  & \hat{\bm{m}}
	)
\end{align}
where \(\hat{\bm{m}}_{D} = v\bm{Y}_{\nu}/\sqrt{2}\). The neutrino mass matrix is diagonalized
using Takagi diagonalization with a unitary matrix \(\bm{\Omega}\). The diagonalization condition
is
\begin{align}\label{eqn:DiagCond}
	\bm{\Omega}^{T}\hat{\bm{M}}\bm{\Omega} & = m^{i}_{\nu}\delta_{ij}, &  & (\text{no sum over } i)
\end{align}
where \(m^{i}_{\nu}\) are the masses of the neutrino mass eigenstates. It is convinient to
write \(\bm{\Omega}\) as
\begin{align}\label{eqn:OmegaDef}
	\bm{\Omega} & = \mqty(\OmegaVVb & \OmegaVNb \\ \OmegaNVb & \OmegaNNb)
\end{align}
where \(\OmegaVVb\) is a \(3\times3\) matrix, \(\OmegaVNb\) is a \(3\times n\) matrix,
\(\OmegaNVb\) is a \(n\times3\) matrix and \(\OmegaNNb\) is a \(n\times n\) matrix.
The neutrino eigenstates are related to the gauge eigenstates through:
\begin{align}
	\hat{\nu}_{i}  & = \qty(\OmegaVVb)^{ij}\nu_j + \qty(\OmegaVNb)^{ij}\rhn_j \\
	\hat{\rhn}_{i} & = \qty(\OmegaNVb)^{ij}\nu_j + \qty(\OmegaNNb)^{ij}\rhn_j
\end{align}
By \ref{eqn:DiagCond}, we find that the block matrices satisfy the following conditions:
\begin{align}
	\bm{m}_{\nu}       & =
	\OmegaVVb^{T}\hat{\bm{m}}_{D}\OmegaNVb+\OmegaNVb^{T}\hat{\bm{m}}^{T}_{D}\OmegaVVb+\OmegaNVb^{T}\hat{\bm{m}}\OmegaNVb \\
	\bm{0}_{3\times n} & =
	\OmegaNVb^{T}\hat{\bm{m}}^{T}_{D}\OmegaVNb+\OmegaVVb^{T}\hat{\bm{m}}_{D}\OmegaNNb+\OmegaNVb^{T}\hat{\bm{m}}\OmegaNNb \\
	\bm{0}_{n\times 3} & =
	\OmegaVNb^{T}\hat{\bm{m}}_{D}\OmegaNVb
	+\OmegaNNb^{T}\hat{\bm{m}}^{T}_{D}\OmegaVVb
	+\OmegaNNb^{T} \hat{\bm{m}}\OmegaNVb                                                                                 \\
	\bm{m}_{\rhn}      & =
	\OmegaVNb^{T}\hat{\bm{m}}_{D}\OmegaNNb
	+\OmegaNNb^{T}\hat{\bm{m}}^{T}_{D}\OmegaVNb
	+\OmegaNNb^{T} \hat{\bm{m}}\OmegaNNb
\end{align}
where \(\bm{m}_{\nu}\) is a diagonal \(3\times3\) mass matrix and \(\bm{m}_{\rhn}\) is a
\(n\times n\) diagonal mass matrix. These conditions can be flipped to obtain \(\hat{\bm{m}}_{D}\) and \(\hat{\bm{m}}\)
in terms of the mixing and mass matrices:
\begin{align}
	\hat{\bm{m}}_{D}  & = \OmegaVVb^{*}\bm{m}_{\nu}\OmegaNVb^{\dagger} + \OmegaVNb^{*}\bm{m}_{\rhn}\OmegaNNb^{\dagger} \\
	\hat{\bm{m}}      & = \OmegaNVb^{*}\bm{m}_{\nu}\OmegaNVb^{\dagger} + \OmegaNNb^{*}\bm{m}_{\rhn}\OmegaNNb^{\dagger} \\
	\bm{0}_{3\times3} & = \OmegaVVb^{*}\bm{m}_{\nu}\OmegaVVb^{\dagger} + \OmegaVNb^{*}\bm{m}_{\rhn}\OmegaVNb^{\dagger}
\end{align}

By unitarity, we have:
\begin{align}
	\bm{1}_{3\times3}  & = \OmegaVVb^{\dagger}\OmegaVVb+\OmegaVNb^{\dagger}\OmegaNVb \\
	\bm{0}_{3\times n} & = \OmegaVVb^{\dagger}\OmegaVNb+\OmegaNVb^{\dagger}\OmegaNNb \\
	\bm{0}_{n\times3}  & = \OmegaVNb^{\dagger}\OmegaVVb+\OmegaNNb^{\dagger}\OmegaNVb \\
	\bm{1}_{n\times n} & = \OmegaNVb^{\dagger}\OmegaVNb+\OmegaNNb^{\dagger}\OmegaNNb
\end{align}

The charged lepton mass matrix is diagonalized in a slightly different fashion (since the mass matrix
is no longer a complex symmetric matrix), which we review here. The charge lepton
yukawa interaction yields the following mass terms:
\begin{align}
	\cL_{\ell,\mathrm{mass}}\supset -\frac{v}{\sqrt{2}}\bm{Y}_{\ell}^{ij}
	\hat{\ell}_{i}\hat{\bar{\ell}}_{j} + \mathrm{c.c.}
\end{align}
where \(\hat{\bar{\ell}}_{i}\) is the gauge eigenstate for the right-handed charged leptons.
To diagonalize \(v\bm{Y}_{\ell}/\sqrt{2}\), we employ singular-value decomposition. Apply
a unitary matrix \(\bm{L}_{\ell}\) and \(\bm{R}_{\ell}\) to the left-handed and right-handed
charged leptons, respectively. Then, we require that:
\begin{align}
	\frac{v}{\sqrt{2}}
	\qty(\bm{L}^T\bm{Y}_{\ell}\bm{R})^{ij}
	= m_{i}\delta_{ij}
	(\text{no sum over } i)
\end{align}
The masses \(m_{i}\) can be obtained by compute the positive square roots of
\(\bm{Y}_{\ell}^{\dagger}\bm{Y}_{\ell}\) (which is a Hermitian matrix.) From now on,
we will assume that the charge leptons rotations have been performed. We will also rotate
the left-handed neutrinos by \(\bm{L}_{\ell}\) and redefine the neutrino Yukawa such
that \(\bm{Y}_{\nu}\to \bm{L}_{\ell}\bm{Y}_{\nu}\).
