# Supplementary material for: Sterile Neutrinos from Dark Matter: A $\nu$ Nightmare?
Source: arXiv:2211.05996 source file (2022-11-11)
Supplement: Supplementary file 9 [file single_rhn.tex]

Here we specialize the above discussion to the case with a single RH neutrino (i.e
\(n=1\)). In this case, the neutrino mass matrix takes the form
\begin{align}
	\hat{\bm{M}} = \mqty(
	0             & 0               & 0                & \hat{m}_{D,e}    \\
	0             & 0               & 0                & \hat{m}_{D,\mu}  \\
	0             & 0               & 0                & \hat{m}_{D,\tau} \\
	\hat{m}_{D,e} & \hat{m}_{D,\mu} & \hat{m}_{D,\tau} & \mu              \\
	)
\end{align}
where \(\hat{m}_{D,\ell} = v y_{\ell}/\sqrt{2}\). For now, we assume the \(\hat{m}_{D,\ell}\)
are real (we relax this later.) The eigenvalues of
\(\hat{\bm{M}}\) are:
\begin{align}
	m_{1} & = m_{2} = 0                                     \\
	m_{3} & = \frac{\mu}{2}\qty(\sqrt{1 + 2\epsilon^{2}}-1) \\
	m_{4} & = \frac{\mu}{2}\qty(\sqrt{1 + 2\epsilon^{2}}+1)
\end{align}
where \(\epsilon=vy/\mu\) and \(y^{2}=y_{e}^{2}+y_{\mu}^{2}+y_{\tau}^{2}\).
Then mass eigenstates are:
\begin{align}
	\nu_{1} & = \frac{1}{\sqrt{y^{2}_{e}\qty(y^{2}_{\mu} + y^{2}_{\tau})}}
	\mqty(0                                                                               \\
	-y_{e}y_{\tau}                                                                        \\
	y_{e}y_{\mu}                                                                          \\
	0),     &
	\nu_{2} & = \frac{1}{\sqrt{y^{2}y_{\tau}^2y_{\mu}^{2}\qty(y_{\mu}^{2}+y_{\tau}^{2})}}
	\mqty(
	-y_{\mu}y_{\tau}\qty(y_{\mu}^{2}+y_{\tau}^{2})                                        \\
	y_{e}y^{2}_{\mu}y_{\tau}                                                              \\
	y_{e}y_{\mu}y^{2}_{\tau}                                                              \\
	0)                                                                                    \\
	\nu_{3} & = \frac{i}{\sqrt{2m^{2}_{3} + v^2y^2}}
	\mqty(
	v y_{e}                                                                               \\
	v y_{\mu}                                                                             \\
	v y_{\tau}                                                                            \\
	-\sqrt{2}m_{3}
	),      &
	\nu_{4} & = \frac{1}{\sqrt{2m^{2}_{4} + v^2y^2}}
	\mqty(
	v y_{e}                                                                               \\
	v y_{\mu}                                                                             \\
	v y_{\tau}                                                                            \\
	-\sqrt{2}m_{4}
	)
\end{align}
with \(\Omega\) being the matrix with the eigenstates as columns. If we set
\(y_{\tau} = y\) and \(y_{e}=y_{\mu}=0\), we \(\Omega\) is (which we will denote
as \(\Omega_{0}\))
\begin{align}
	\Omega_{0}
	  & =
	\mqty(
	1 & 0 & 0                            & 0                           \\
	0 & 1 & 0                            & 0                           \\
	0 & 0 & i\sqrt{\frac{m_4}{m_4+m_3}}  & \sqrt{\frac{m_3}{m_4+m_3}}  \\
	0 & 0 & -i\sqrt{\frac{m_3}{m_4+m_3}} & \sqrt{\frac{m_4}{m_4+m_3}})
\end{align}
If we define a mixing angle \(\theta\) such that:
\begin{align}
	\cos\theta & = \sqrt{\frac{m_4}{m_4+m_3}}, &
	\sin\theta & = \sqrt{\frac{m_3}{m_4+m_3}}
\end{align}
then \(\tan^2\theta = m_{3}/m_{4}\). We can therefore define all the parameters in
terms of the mixing angle and the heavy mass. Let \(m_{\nu}=m_{3}\) and
\(m_{4} = m_{\rhn}\). Then,
\begin{align}
	m_{\nu} & = m_{\rhn}\tan^2\theta,                 &
	y       & = \frac{\sqrt{2}m_{\rhn}}{v}\tan\theta, &
	\mu     & = m_{\rhn}\qty(1-\tan^2\theta)
\end{align}
In the case where \(y_{e},y_{\mu}\) and \(y_{\tau}\) are all non-zero, then we
first perform a rotation such that we remove \(y_{e}\) and \(y_{\mu}\). This is
done using a rotation matrix \(R\) such that:
\begin{align}
	R^{T}\hat{\bm{M}}R =
	\mqty(
	0 & 0 & 0                  & 0                  \\
	0 & 0 & 0                  & 0                  \\
	0 & 0 & 0                  & \sqrt{v}y/\sqrt{2} \\
	0 & 0 & \sqrt{v}y/\sqrt{2} & \mu                \\
	)
\end{align}
To achive this, we use the following rotation matrix:
\begin{align}
	R = \mqty(
	\cos\alpha\cos\beta & -\sin\beta & \cos\beta\sin\alpha & 0 \\
	\cos\alpha\sin\beta & \cos\beta  & \sin\alpha\sin\beta & 0 \\
	-\sin\alpha         & 0          & \cos\alpha          & 0 \\
	0                   & 0          & 0                   & 1
	)
\end{align}
where \(\alpha\) and \(\beta\) are such that
\begin{align}
	y_{e}    & = y\cos\beta\sin\alpha, &
	y_{\mu}  & = y\sin\beta\sin\alpha, &
	y_{\tau} & = y\cos\alpha,          &
\end{align}
Then, \(R^{T}\hat{\bm{M}}R\) is diagonalized using the above \(\Omega_{0}\). That
is, \(\Omega^{T}_{0}R^{T}\hat{\bm{M}}R\Omega_{0}\) is diagonal. And therefore, we
identify the full roation matrix as \(\Omega = R\Omega_{0}\), which is:
\begin{align}
	\Omega = \mqty(
	\cos\alpha\cos\beta & -\sin\beta & i \sin\alpha\cos\beta\cos\theta & \sin\alpha\cos\beta\sin\theta \\
	\cos\alpha\sin\beta & \cos\beta  & i \sin\alpha\sin\beta\cos\theta & \sin\alpha\sin\beta\sin\theta \\
	-\sin\alpha         & 0          & i \cos\alpha\cos\theta          & \cos\alpha\sin\theta          \\
	0                   & 0          & -i \sin\theta                   & \cos\theta                    \\
	)
\end{align}

Lastly, we let the \(y_{\ell}\) be complex. In this case, we need to remove the
phases before applying the above \(\Omega\). We can write
\(\tilde{y}_{\ell}= y_{\ell}e^{i\delta_{\ell}}\). We can rephase the RH-Neutrino field
to absorb the phase of \(\mu\). Thus, the mass matrix with complex Yukawas is:
\begin{align}
	\hat{\bm{M}} = \frac{v}{\sqrt{2}}\mqty(
	0             & 0               & 0                & \tilde{y}_{e}    \\
	0             & 0               & 0                & \tilde{y}_{\mu}  \\
	0             & 0               & 0                & \tilde{y}_{\tau} \\
	\tilde{y}_{e} & \tilde{y}_{\mu} & \tilde{y}_{\tau} & \sqrt{2}\mu/v    \\
	)
\end{align}
Applying a phase matrix \(\bm{P}\) to the mass matrix as \(\bm{P}^{T}\hat{\bm{M}}\bm{P}\)
removes all of the phases. Here, the matrix \(\bm{P}\) is given by:
\begin{align}
	\bm{P}
	=
	\mqty(\dmat{
		e^{-i\delta_{e}} ,
		e^{-i\delta_{\mu}},
		e^{-i\delta_{\tau}},
		1
	})
\end{align}
Thus, the full mixing matrix \(\Omega\) for the neutrinos is given by the following product of
rotations and phases:
\begin{align}
	\Omega      & =
	\mqty(\dmat{
		e^{-i\delta_{e}} ,
		e^{-i\delta_{\mu}},
		e^{-i\delta_{\tau}},
		1
	})
	\mqty(
	\dmat{
	\cos\beta   & -\sin\beta                   \\
	\sin\beta   & \cos\beta,1,1}
	)                                          \\
	            & \quad\times
	\mqty(\dmat{
	\cos\alpha  &                & \sin\alpha  \\
	            & 1              &             \\
	-\sin\alpha &                & \cos\alpha,
		1
	})
	\mqty(\dmat{
		1,1,
	\cos\theta  & \sin\theta                   \\
	-\sin\theta & \cos\theta                   \\
	})
	\mqty(\dmat{1,1,e^{i\pi/2},1})
\end{align}
If we take the 3 angles and the heavy neutrino mass as our parameters, the
yukawas and majorana mass are given by:
\begin{align}
	\tilde{y}_{e}    & =\frac{\sqrt{2}m_{\rhn}}{v}\tan\theta\cos\beta\sin\alpha e^{i\delta_{e}},   &
	\tilde{y}_{\mu}  & =\frac{\sqrt{2}m_{\rhn}}{v}\tan\theta\sin\beta\sin\alpha e^{i\delta_{\mu}},   \\
	\tilde{y}_{\tau} & =\frac{\sqrt{2}m_{\rhn}}{v}\tan\theta\cos\alpha e^{i\delta_{\tau}},         &
	\mu              & = m_{\rhn}(1-\tan^2\theta)
\end{align}
and the light neutrino mass is \(m_{\nu} = m_{\rhn}\tan^2\theta\). Additionally, the
PMNS matrices are:
\begin{align}
	\bm{\cK}_{L}
	                                      &
	=
	\mqty(
	e^{-i\delta_{e}}\cos\alpha\cos\beta   &
	-e^{-i\delta_{e}}\sin\beta            &
	i \sin\alpha\cos\beta\cos\theta                   \\
	%e^{-i\delta_{e}}\sin\alpha\cos\beta\sin\theta                             \\
	%----
	e^{-i\delta_{\mu}}\cos\alpha\sin\beta &
	e^{-i\delta_{\mu}}\cos\beta           &
	i e^{-i\delta_{\mu}}\sin\alpha\sin\beta\cos\theta \\
	%& e^{-i\delta_{\mu}}\sin\alpha\sin\beta\sin\theta \\
	%----
	-e^{-i\delta_{\tau}}\sin\alpha        &
	0                                     &
	i e^{-i\delta_{\tau}}\cos\alpha\cos\theta
	%& \cos\alpha\sin\theta          \\
	)                                                 \\
	\bm{\cK}_{R}
	                                      &
	=
	\mqty(
	%e^{-i\delta_{e}}\cos\alpha\cos\beta   &
	%-e^{-i\delta_{e}}\sin\beta            &
	%i \sin\alpha\cos\beta\cos\theta                   \\
	e^{-i\delta_{e}}\sin\alpha\cos\beta\sin\theta     \\
	%----
	%e^{-i\delta_{\mu}}\cos\alpha\sin\beta &
	%e^{-i\delta_{\mu}}\cos\beta           &
	%i e^{-i\delta_{\mu}}\sin\alpha\sin\beta\cos\theta \\
	e^{-i\delta_{\mu}}\sin\alpha\sin\beta\sin\theta   \\
	%----
	%-e^{-i\delta_{\tau}}\sin\alpha        &
	%0                                     &
	%i e^{-i\delta_{\tau}}\cos\alpha\cos\theta
	\cos\alpha\sin\theta                              \\
	)
\end{align}

In the above parameterization, we can see that cases of the RH-neutrino mixing with only
a single LH-neutrino are:
\begin{align}
	\text{electron} & : & \beta & =0,                 & \alpha & =\pi/2, \\
	\text{muon}     & : & \beta & =\pi/2,             & \alpha & =\pi/2, \\
	\text{tau}      & : & \beta & =\mathrm{anything}, & \alpha & =0
\end{align}
