# Supplementary material for: Sterile Neutrinos from Dark Matter: A $\nu$ Nightmare?
Source: arXiv:2211.05996 source file (2022-11-11)
Supplement: Supplementary file 10 [file chipt_two_body.tex]

\subsubsection{\texorpdfstring{\(\rhn_{i}\to\nu_{j}\pi^{0},\nu_{j}\eta\)}{RH-Neutrino to LH-Neutrino and Neutral Pion}}

The relavent interactions for \(\rhn_{i}\to\nu_{j}\pi^{0}\) stem from
\begin{align}
    \cL_{4F} & = -\frac{4\gf\fpi}{2\cw^{2}\sqrt{2}}\qty(\partial_{\mu}\piz)
    \qty(\qty(\OmegaVVb^{\dagger}\OmegaVNb)^{ij}
    \nu_{i}^{\dagger}
    \bar{\sigma}_{\mu}
    \rhn_{j}
    +\qty(\OmegaVNb^{\dagger}\OmegaVVb)^{ij}\rhn_{i}^{\dagger}
    \bar{\sigma}_{\mu}
    \nu_{j}
    )
\end{align}
Thus, the amplitude is given by:
\begin{align}
    i\cM\qty(\rhn_{i}\to\nu_{j}\pi^{0})
    =
    -i\frac{\sqrt{2}\gf\fpi}{\cw^{2}}\qty(i p^{\mu}_{\piz})
    \qty[
    gx^{\dagger}_{\nu}\bar{\sigma}_{\mu}x_{\rhn}
    -
    g^{*}y^{\dagger}_{\rhn}\bar{\sigma}_{\mu}y_{\nu}
    ]
\end{align}
where \(g\equiv \qty(\OmegaVVb^{\dagger}\OmegaVNb)^{ij}\).
Squaring and summing over spins yields:
\begin{align}
    \frac{1}{2}\sum_{\mathrm{spins}}\qty|\cM\qty(\rhn_{i}\to\nu_{j}\pi^{0})|^{2}
     & =
    \frac{2\gf^{2}\fpi^{2}}{\cw^{4}}
    \bigg{[}
    |g|^{2}\qty(\qty(m_{\rhn_{i}}^{2}-m_{\nu_{j}}^{2})^{2}
    - m_{\piz}^{2}\qty(m_{\rhn_{i}}^{2}+m_{\nu_{j}}^{2})) \\
     & \qquad\qquad\qquad
    -4\Re(g^2)m_{\rhn_{i}}m_{\nu_{j}}m_{\piz}^{2}
    \bigg{]}\notag
\end{align}
and thus, the partial width is:
\begin{align}
    \Gamma\qty(\rhn_{i}\to\nu_{j}\pi^{0})
    =
    \frac{\gf^{2}\fpi^{2}m^{3}_{\rhn_{i}}}{8\pi \cw^{4}}
    \lambda^{1/2}(1,\beta_{\nu_{j}}^2,\beta_{\pi}^{2})
     &
    \bigg{[}
    |g|^{2}\qty(\qty(1-\beta_{\nu_{j}}^{2})^{2}
    - \beta_{\piz}^{2}\qty(1+\beta_{\nu_{j}}^{2})) \\
     & \quad
    -4\Re(g^2)\beta_{\nu_{j}}\beta_{\piz}^{2}
    \bigg{]}\notag
\end{align}
The result for \(\rhn_{i}\to\nu_{j}\eta\) is identical but has an extra factor of
\(1/3\)
\begin{align}
    \Gamma\qty(\rhn_{i}\to\nu_{j}\eta)
    =
    \frac{\gf^{2}\fpi^{2}m^{3}_{\rhn_{i}}}{24\pi \cw^{4}}
    \lambda^{1/2}(1,\beta_{\nu_{j}}^2,\beta_{\eta}^{2})
     &
    \bigg{[}
    |g|^{2}\qty(\qty(1-\beta_{\nu_{j}}^{2})^{2}
    - \beta_{\eta}^{2}\qty(1+\beta_{\nu_{j}}^{2})) \\
     & \quad
    -4\Re(g^2)\beta_{\nu_{j}}\beta_{\eta}^{2}
    \bigg{]}\notag
\end{align}

\subsubsection{\texorpdfstring{\(\rhn_{i}\to\ell_{j}\pip,\ell_{j}\kp\)}{RH-Neutrino to Charged Lepton and Charged Pion}}

The relavent interactions for \(\rhn_{i}\to\ell_{j}\pip\) stem from
\begin{align}
    \cL_{4F} & = -2\gf\fpi\vud\qty(\partial_{\mu}\pim)
    \qty(\OmegaVNb)^{ji}
    \ell_{j}^{\dagger}
    \bar{\sigma}_{\mu}
    \rhn_{i}
\end{align}
Thus, the amplitude is given by:
\begin{align}
    i\cM\qty(\rhn_{i}\to\ell_{j}\pip)
    =
    -2g\gf\fpi\vud\qty(ip_{\pip})
    x^{\dagger}_{\ell}\bar{\sigma}_{\mu}x_{\rhn}
\end{align}
where \(g\equiv \qty(\OmegaVNb)^{ji}\).
Squaring and summing over spins yields:
\begin{align}
    \frac{1}{2}\sum_{\mathrm{spins}}\qty|\cM\qty(\rhn_{i}\to\ell_{j}\pip)|^{2}
     & =
    2\qty|g|^{2}\gf^{2}\fpi^{2}\qty|\vud|^{2}
    \qty[\qty(m_{\rhn_{i}}^{2}-m_{\ell_{j}}^{2})^{2}
        - m_{\pip}^{2}\qty(m_{\rhn_{i}}^{2}+m_{\ell_{j}}^{2})]
\end{align}
and thus, the partial width is:
\begin{align}
    \Gamma\qty(\rhn_{i}\to\ell_{j}\pip)
    =
    \frac{\qty|g|^{2}\gf^{2}\fpi^{2}\qty|\vud|^{2}m^{3}_{\rhn_{i}}}{8\pi}
    \lambda^{1/2}(1,\beta_{\ell}^2,\beta_{\pip}^{2})
    \qty[\qty(1-\beta_{\ell_{j}}^{2})^{2}
        - \beta_{\pip}^{2}\qty(1+\beta_{\ell_{j}}^{2})]
\end{align}
The result for \(\rhn_{i}\to\ell_{j}K^{+}\) is obtained from the above with
the replacements \(V_{ud}\to V_{us}\) and \(\beta_{\pip}\to\beta_{\kp}\)
\begin{align}
    \Gamma\qty(\rhn_{i}\to\ell_{j}\kp)
    =
    \frac{\qty|g|^{2}\gf^{2}\fpi^{2}\qty|\vus|^{2}m^{3}_{\rhn_{i}}}{8\pi}
    \lambda^{1/2}(1,\beta_{\ell}^2,\beta_{\kp}^{2})
    \qty[\qty(1-\beta_{\ell_{j}}^{2})^{2}
        - \beta_{\kp}^{2}\qty(1+\beta_{\ell_{j}}^{2})]
\end{align}
