# Supplementary material for: Sterile Neutrinos from Dark Matter: A $\nu$ Nightmare?
Source: arXiv:2211.05996 source file (2022-11-11)
Supplement: Supplementary file 11 [file ew_n_to_ell_w.tex]

The amplitude for \(\rhn_{i}(P) \to W^{+}(p_{W}) + \ell_{j}(p_{\ell})\) is given by:
\begin{align}
    \cM & = -i\frac{e}{\sqrt{2}s_{W}}G_{ij} x^{\dagger}(p_{\ell})\bar{\sigma}_{\mu}x(P)
\end{align}
where \(G_{ij} = \qty(\OmegaVNb)_{ij}\). Squaring and summing
over spins, we find:
\begin{align}
    \frac{1}{2}\sum_{\mathrm{spins}}\qty|\cM|^2
     & =
    \frac{e^{2}\qty|\OmegaVNb^{ij}|^2}{4M_{W}^{2}}
    \qty(
    \qty(m_{\rhn_{i}}-m_{\ell_{j}})^{2}
    +\qty(m^{2}_{\rhn_{i}}+m^{2}_{\ell_{j}})M_{W}^{2}
    -2M_{W}^{4}
    )
\end{align}
The partial width is therefore:
% prefactor \lambda^{1/2}(m^{2}_{\rhn_{i}},m_{1}^2,m_{2}^{2}) / (16\pi m^{3}_{\rhn^{2}_{i}})
\begin{align}
    \Gamma(\rhn_{i}\to \ell_{j}W^{+})
     & =
    \frac{e^{2}\lambda^{1/2}(m^{2}_{\rhn_{i}},m_{\ell_{j}}^2,M_{W}^{2})}{64\pi M^{2}_{W}m^{3}_{\rhn^{2}_{i}}}
    \qty|\OmegaVNb^{ij}|^2
    \qty(
    \qty(m_{\rhn_{i}}-m_{\ell_{j}})^{2}
    +\qty(m^{2}_{\rhn_{i}}+m^{2}_{\ell_{j}})M_{W}^{2}
    -2M_{W}^{4}
    )\notag                                               \\
     & \quad\times\theta(m_{\rhn_{i}}-m_{\ell_{j}}-M_{W})
\end{align}
