# Supplementary material for: Sterile Neutrinos from Dark Matter: A $\nu$ Nightmare?
Source: arXiv:2211.05996 source file (2022-11-11)
Supplement: Supplementary file 12 [file ew_n_to_nu_gamma.tex]

In two component spinor notation, there are either 6 or 12 diagrams contributing to
\(\rhn_{i}\to\nu_{j}\gamma\) at one loop, depending on the gauge used. These are shown in
\FigRef{fig:n_to_nu_gamma_w} and \FigRef{fig:n_to_nu_gamma_ell}.

\begin{figure}[ht!]
    \centering
    \begin{subfigure}[b]{0.45\linewidth}
        \begin{tikzpicture}
            \begin{feynman}
                \vertex (i1)  {\(\rhn_{i}\)};
                \vertex[right=1cm of i1] (v1) ;
                \vertex[right=1cm of v1] (g1) ;
                \vertex[right=1cm of g1] (v2) ;
                \vertex[above=1cm of g1] (v3) ;
                \vertex[right=1cm of v2] (o1) {\(\nu_{j}\)};
                \vertex[above=1cm of v3] (g2) ;
                \vertex[right=1cm of g2] (o2) {\(\gamma\)};
                \diagram*{
                (i1) -- [fermion] (v1) -- [fermion,edge label=\(\ell_{k}\)](v2) -- [fermion](o1);
                (v1) -- [charged boson,quarter left,looseness=1.0,edge label=\(W^{+}\)] (v3) -- [charged boson,quarter left,looseness=1.0] (v2);
                (v3) -- [boson] (o2);
                };
            \end{feynman}
        \end{tikzpicture}
        \caption{}
    \end{subfigure}
    \begin{subfigure}[b]{0.45\linewidth}
        \begin{tikzpicture}
            \begin{feynman}
                \vertex (i1)  {\(\rhn_{i}\)};
                \vertex[right=1cm of i1] (v1) ;
                \vertex[right=1cm of v1] (g1) ;
                \vertex[right=1cm of g1] (v2) ;
                \vertex[above=1cm of g1] (v3) ;
                \vertex[right=1cm of v2] (o1) {\(\nu_{j}\)};
                \vertex[above=1cm of v3] (g2) ;
                \vertex[right=1cm of g2] (o2) {\(\gamma\)};
                \diagram*{
                (o1) -- [fermion] (v2) -- [fermion](v1) -- [fermion](i1);
                (v1) -- [anti charged boson,quarter left,looseness=1.0] (v3) -- [anti charged boson,quarter left,looseness=1.0] (v2);
                (v3) -- [boson] (o2);
                };
            \end{feynman}
        \end{tikzpicture}
        \caption{}
    \end{subfigure}
    \begin{subfigure}[b]{0.45\linewidth}
        \begin{tikzpicture}
            \begin{feynman}
                \vertex (i1)  {\(\rhn_{i}\)};
                \vertex[right=1cm of i1] (v1) ;
                \vertex[right=1cm of v1] (g1) ;
                \vertex[right=1cm of g1] (v2) ;
                \vertex[above=1cm of g1] (v3) ;
                \vertex[right=1cm of v2] (o1) {\(\nu_{j}\)};
                \vertex[above=1cm of v3] (g2) ;
                \vertex[right=1cm of g2] (o2) {\(\gamma\)};
                \diagram*{
                (i1) -- [fermion] (v1) -- [anti fermion,edge label=\(\ell_{k}\)](v2) -- [fermion](o1);
                (v1) -- [anti charged scalar,quarter left,looseness=1.0,edge label=\(G^{+}\)] (v3) -- [anti charged scalar,quarter left,looseness=1.0] (v2);
                (v3) -- [boson] (o2);
                };
            \end{feynman}
        \end{tikzpicture}
        \caption{}
    \end{subfigure}
    \begin{subfigure}[b]{0.45\linewidth}
        \begin{tikzpicture}
            \begin{feynman}
                \vertex (i1)  {\(\rhn_{i}\)};
                \vertex[right=1cm of i1] (v1) ;
                \vertex[right=1cm of v1] (g1) ;
                \vertex[right=1cm of g1] (v2) ;
                \vertex[above=1cm of g1] (v3) ;
                \vertex[right=1cm of v2] (o1) {\(\nu_{j}\)};
                \vertex[above=1cm of v3] (g2) ;
                \vertex[right=1cm of g2] (o2) {\(\gamma\)};
                \diagram*{
                (o1) -- [fermion] (v2) -- [anti fermion](v1) -- [fermion](i1);
                (v1) -- [charged scalar,quarter left,looseness=1.0] (v3) -- [charged scalar,quarter left,looseness=1.0] (v2);
                (v3) -- [boson] (o2);
                };
            \end{feynman}
        \end{tikzpicture}
        \caption{}
    \end{subfigure}
    \caption{Diagrams contributing to \(\rhn_{i}\to\nu_{j}\gamma\) with photon
        emission from \(W\)-boson.}
    \label{fig:n_to_nu_gamma_w}
\end{figure}

\begin{figure}[ht!]
    \centering
    \begin{subfigure}[b]{0.45\linewidth}
        \begin{tikzpicture}
            \begin{feynman}
                \vertex (i1)  {\(\rhn_{i}\)};
                \vertex[right=1cm of i1] (v1) ;
                \vertex[right=1cm of v1] (v2) ;
                \vertex[right=1cm of v2] (v3) ;
                \vertex[right=1cm of v3] (o1) {\(\nu_{j}\)};
                \vertex[below=1cm of v2] (g1) ;
                \vertex[right=1cm of g1] (o2) {\(\gamma\)};
                \diagram*{
                (i1) -- [fermion] (v1) -- [fermion,edge label'=\(\ell_{k}\)](v2) -- [fermion](v3) -- [fermion](o1);
                (v1) -- [charged boson,half left,looseness=1.5,edge label=\(W^{+}\)] (v3) ;
                (v2) -- [boson] (o2);
                };
            \end{feynman}
        \end{tikzpicture}
        \caption{}
    \end{subfigure}
    \begin{subfigure}[b]{0.45\linewidth}
        \begin{tikzpicture}
            \begin{feynman}
                \vertex (i1)  {\(\rhn_{i}\)};
                \vertex[right=1cm of i1] (v1) ;
                \vertex[right=1cm of v1] (v2) ;
                \vertex[right=1cm of v2] (v3) ;
                \vertex[right=1cm of v3] (o1) {\(\nu_{j}\)};
                \vertex[below=1cm of v2] (g1) ;
                \vertex[right=1cm of g1] (o2) {\(\gamma\)};
                \diagram*{
                (i1) -- [anti fermion] (v1) -- [anti fermion](v2) -- [anti fermion](v3) -- [anti fermion](o1);
                (v1) -- [anti charged boson,half left,looseness=1.5] (v3) ;
                (v2) -- [boson] (o2);
                };
            \end{feynman}
        \end{tikzpicture}
        \caption{}
    \end{subfigure}
    \begin{subfigure}[b]{0.45\linewidth}
        \begin{tikzpicture}
            \begin{feynman}
                \vertex (i1)  {\(\rhn_{i}\)};
                \vertex[right=1cm of i1] (v1) ;
                \vertex[right=1cm of v1] (v2) ;
                \vertex[right=1cm of v2] (v3) ;
                \vertex[right=1cm of v3] (o1) {\(\nu_{j}\)};
                \vertex[below=1cm of v2] (g3) ;
                \vertex[right=1cm of g3] (o2) {\(\gamma\)};
                \diagram*{
                (i1) -- [fermion] (v1) -- [majorana](v2) -- [anti majorana] (v3) -- [fermion](o1);
                (v1) -- [charged boson,half left,looseness=1.5] (v3) ;
                (v2) -- [boson] (o2);
                };
            \end{feynman}
        \end{tikzpicture}
        \caption{}
    \end{subfigure}
    \begin{subfigure}[b]{0.45\linewidth}
        \begin{tikzpicture}
            \begin{feynman}
                \vertex (i1)  {\(\rhn_{i}\)};
                \vertex[right=1cm of i1] (v1) ;
                \vertex[right=1cm of v1] (v2) ;
                \vertex[right=1cm of v2] (v3) ;
                \vertex[right=1cm of v3] (o1) {\(\nu_{j}\)};
                \vertex[below=1cm of v2] (g3) ;
                \vertex[right=1cm of g3] (o2) {\(\gamma\)};
                \diagram*{
                (i1) -- [anti fermion] (v1) -- [anti majorana](v2) -- [majorana] (v3) -- [anti fermion](o1);
                (v1) -- [anti charged boson,half left,looseness=1.5] (v3) ;
                (v2) -- [boson] (o2);
                };
            \end{feynman}
        \end{tikzpicture}
        \caption{}
    \end{subfigure}
    \begin{subfigure}[b]{0.45\linewidth}
        \begin{tikzpicture}
            \begin{feynman}
                \vertex (i1)  {\(\rhn_{i}\)};
                \vertex[right=1cm of i1] (v1) ;
                \vertex[right=1cm of v1] (v2) ;
                \vertex[right=1cm of v2] (v3) ;
                \vertex[right=1cm of v3] (o1) {\(\nu_{j}\)};
                \vertex[below=1cm of v2] (g1) ;
                \vertex[right=1cm of g1] (o2) {\(\gamma\)};
                \diagram*{
                (i1) -- [fermion] (v1) -- [anti fermion,edge label'=\(\ell_{k}\)](v2) -- [anti fermion](v3) -- [fermion](o1);
                (v1) -- [anti charged scalar,half left,looseness=1.5,edge label=\(G^{+}\)] (v3) ;
                (v2) -- [boson] (o2);
                };
            \end{feynman}
        \end{tikzpicture}
        \caption{}
    \end{subfigure}
    \begin{subfigure}[b]{0.45\linewidth}
        \begin{tikzpicture}
            \begin{feynman}
                \vertex (i1)  {\(\rhn_{i}\)};
                \vertex[right=1cm of i1] (v1) ;
                \vertex[right=1cm of v1] (v2) ;
                \vertex[right=1cm of v2] (v3) ;
                \vertex[right=1cm of v3] (o1) {\(\nu_{j}\)};
                \vertex[below=1cm of v2] (g1) ;
                \vertex[right=1cm of g1] (o2) {\(\gamma\)};
                \diagram*{
                (i1) -- [anti fermion] (v1) -- [fermion](v2) -- [fermion](v3) -- [anti fermion](o1);
                (v1) -- [charged scalar,half left,looseness=1.5] (v3) ;
                (v2) -- [boson] (o2);
                };
            \end{feynman}
        \end{tikzpicture}
        \caption{}
    \end{subfigure}
    \begin{subfigure}[b]{0.45\linewidth}
        \begin{tikzpicture}
            \begin{feynman}
                \vertex (i1)  {\(\rhn_{i}\)};
                \vertex[right=1cm of i1] (v1) ;
                \vertex[right=1cm of v1] (v2) ;
                \vertex[right=1cm of v2] (v3) ;
                \vertex[right=1cm of v3] (o1) {\(\nu_{j}\)};
                \vertex[below=1cm of v2] (g3) ;
                \vertex[right=1cm of g3] (o2) {\(\gamma\)};
                \diagram*{
                (i1) -- [fermion] (v1) -- [anti majorana](v2) -- [majorana] (v3) -- [fermion](o1);
                (v1) -- [anti charged scalar,half left,looseness=1.5] (v3) ;
                (v2) -- [boson] (o2);
                };
            \end{feynman}
        \end{tikzpicture}
        \caption{}
    \end{subfigure}
    \begin{subfigure}[b]{0.45\linewidth}
        \begin{tikzpicture}
            \begin{feynman}
                \vertex (i1)  {\(\rhn_{i}\)};
                \vertex[right=1cm of i1] (v1) ;
                \vertex[right=1cm of v1] (v2) ;
                \vertex[right=1cm of v2] (v3) ;
                \vertex[right=1cm of v3] (o1) {\(\nu_{j}\)};
                \vertex[below=1cm of v2] (g3) ;
                \vertex[right=1cm of g3] (o2) {\(\gamma\)};
                \diagram*{
                (i1) -- [anti fermion] (v1) -- [majorana](v2) -- [anti majorana] (v3) -- [anti fermion](o1);
                (v1) -- [charged scalar,half left,looseness=1.5] (v3) ;
                (v2) -- [boson] (o2);
                };
            \end{feynman}
        \end{tikzpicture}
        \caption{}
    \end{subfigure}
    \caption{Diagrams contributing to \(\rhn_{i}\to\nu_{j}\gamma\) with photon
        emission from charged lepton. Note diagrams use two-component spinors
        with (c), (d), (g) and (f) representing charged lepton mass insertions.}
    \label{fig:n_to_nu_gamma_ell}
\end{figure}

We will denote the \(W^{+}W^{-}\gamma\) vertex as \(V^{\alpha\beta\mu}(p^{+}_{\alpha},p^{-}_{\beta},p^{\gamma}_{\mu})\),
given by:
\begin{align}
	V_{WW\gamma}^{\alpha\beta\mu}(p^{+}_{\alpha},p^{-}_{\beta},p^{\gamma}_{\mu}) =
	ie\qty[
		g^{\alpha\beta}\qty(p^{-}-p^{+})_{\mu} +
		g^{\alpha\mu}\qty(p^{+}-p^{\gamma})_{\beta} +
		g^{\beta\mu}\qty(p^{\gamma}-p^{-})_{\alpha}
	]
\end{align}
We denote the \(G^{+}G^{-}\gamma\) vertex as \(V^{\mu}(p^{+},p^{-})\), given by:
\begin{align}
	V_{GG\gamma}^{\mu}(p^{+},p^{-}) = ie\qty(p^{+} - p^{-})_{\mu}
\end{align}
Note that \(V_{WW\gamma}^{\alpha\beta\mu}(p^{+}_{\alpha},p^{-}_{\beta},p^{\gamma}_{\mu}) = -V_{WW\gamma}^{\beta\alpha\mu}(p^{-}_{\alpha},p^{+}_{\beta},p^{\gamma}_{\mu})\)
and \(V_{GG\gamma}^{\mu}(p^{+},p^{-}) = - V_{GG\gamma}^{\mu}(p^{-},p^{+})\).
We use \(\Delta\) for a propagator. For example:
\begin{align}
	\Delta^{\mu\nu}_{W}(p) & = \frac{i}{p^2-M_{W}^{2}+i\epsilon}\qty(-g^{\mu\nu} + (1-\xi)\frac{p^{\mu}p^{\nu}}{p^{2}-\xi M_{W}^{2}}) \\
	\Delta^{G}(p)          & = \frac{i}{p^2-\xi M_{W}^{2}+i\epsilon}
\end{align}
In addition, we denote the neutrino interactions as:
\begin{align}
	V^{\mu}_{W\nu_{i}\ell_{j}}  & \equiv A = \frac{e}{\sqrt{2}\sw}\qty(\bm{\cK}_{L})^{ij}\bar{\sigma}_{\mu}     \\
	V^{\mu}_{W\rhn_{i}\ell_{j}} & \equiv B = \frac{e}{\sqrt{2}\sw}\qty(\bm{\cK}_{R})^{ij}\bar{\sigma}_{\mu}     \\
	V_{G\nu_{i}\ell_{j}}        & \equiv \tilde{A} =  \frac{e}{\sqrt{2}\sw}\qty(\hat{\bm{m}}_{D}\OmegaVVb)^{ij} \\
	V_{G\rhn_{i}\ell_{j}}       & \equiv \tilde{B} = \frac{e}{\sqrt{2}\sw}\qty(\hat{\bm{m}}_{D}\OmegaVNb)^{ij}
\end{align}

% ============================================================================
% ---- W-Emission Diagrams ---------------------------------------------------
% ============================================================================

The amplitude of the diagrams with \(W\)-bosons in \FigRef{fig:n_to_nu_gamma_w} are given by
\begin{align}
	i\cA^{(a)}_{1}
	 & =
	-i\qty(A^{*}B)
	\int\frac{\dd[4]{\ell}}{(2\pi)^{4}}
	\frac{x_{\nu}^{\dagger}(q)\bar{\sigma}_{\mu}\qty(\ell\cdot\sigma)\bar{\sigma}_{\nu}x_{\rhn}(p)}{\ell^{2}-m_{\ell_{k}}^{2}} \\
	 & \quad \times
	\Delta^{\nu\rho}_{W}(p-\ell)
	\Delta^{\lambda\mu}_{W}(\ell-q)
	V^{\rho\lambda\alpha}_{WW\gamma}(p-\ell,\ell-q,-k)
	\epsilon^{*}_{\alpha}(k)
	\notag                                                                                                                     \\
	%--------------------------
	i\cA^{(b)}_{1}
	 & =
	i\qty(AB^{*})
	\int\frac{\dd[4]{\ell}}{(2\pi)^{4}}
	\frac{y_{\nu}(q)\sigma_{\mu}\qty(\ell\cdot\bar{\sigma})\sigma_{\nu}y^{\dagger}_{\rhn}(p) }{\ell^{2}-m_{\ell_{k}}^{2}}      \\
	 & \quad \times
	\Delta^{\nu\rho}_{W}(p-\ell)
	\Delta^{\lambda\mu}_{W}(\ell-q)
	V^{\rho\lambda\alpha}_{WW\gamma}(p-\ell,\ell-q,-k)
	\epsilon^{*}_{\alpha}(k)
	\notag
\end{align}

% ============================================================================
% ---- G-Emission Diagrams ---------------------------------------------------
% ============================================================================

The amplitude of the diagrams with Goldstones in \FigRef{fig:n_to_nu_gamma_w} are given by
\begin{align}
	i\cA^{(c)}_{1}
	 & =
	-i\qty(\tilde{A}\tilde{B}^{*})
	\int\frac{\dd[4]{\ell}}{(2\pi)^{4}}
	\frac{x_{\nu}^{\dagger}(q)\qty[\ell\cdot\bar{\sigma}]x_{\rhn}(p)}{\ell^{2}-m_{\ell_{k}}^{2}}
	\\
	 & \quad \times
	\Delta^{G}(p-\ell)
	\Delta^{G}(\ell-q)
	V^{\alpha}_{GG\gamma}(p-\ell,\ell-q)
	\epsilon^{*}_{\alpha}(k)
	\notag          \\
	%--------------------------
	i\cA^{(d)}_{1}
	 & =
	i\qty(\tilde{A}^{*}\tilde{B})
	\int\frac{\dd[4]{\ell}}{(2\pi)^{4}}
	\frac{y_{\nu}(q)\qty[\ell\cdot\sigma]y^{\dagger}_{\rhn}(p)}{\ell^{2}-m_{\ell_{k}}^{2}}
	\\
	 & \quad \times
	\Delta^{G}(p-\ell)
	\Delta^{G}(\ell-q)
	V^{\alpha}_{GG\gamma}(p-\ell,\ell-q)
	\epsilon^{*}_{\alpha}(k)
	\notag
\end{align}

% ============================================================================
% ---- L-Emission Diagrams with W --------------------------------------------
% ============================================================================

The amplitudes for the diagrams with \(W\)-bosons in \FigRef{fig:n_to_nu_gamma_ell} are given by
\begin{align}
	i\cA^{(a)}_{2}
	 & =
	-ieA^{*}B
	\int\frac{\dd[4]{\ell}}{(2\pi)^{4}}
	\frac{
	x_{\nu}^{\dagger}(q)
	\bar{\sigma}_{\mu}
	\qty[\qty(q-\ell)\cdot\sigma]
	\bar{\sigma}_{\alpha}
	\qty[\qty(p-\ell)\cdot\sigma]
	\bar{\sigma}_{\nu}
	x_{\rhn}(p)
	}{
	\qty[\qty(p-\ell)^{2}-m_{\ell_{k}}^{2}]\qty[\qty(q-\ell)^{2}-m_{\ell_{k}}^{2}]
	}
	\Delta^{\mu\nu}_{W}(\ell)
	\epsilon^{*}_{\alpha}(k)
	\\
	%--------------------------
	i\cA^{(b)}_{2}
	 & =
	ieAB^{*}
	\int\frac{\dd[4]{\ell}}{(2\pi)^{4}}
	\frac{
	y_{\nu}(q)
	\sigma_{\mu}
	\qty[\qty(q-\ell)\cdot\bar{\sigma}]
	\sigma_{\alpha}
	\qty[\qty(p-\ell)\cdot\bar{\sigma}]
	\sigma_{\nu}
	y_{\rhn}^{\dagger}(p)
	}{
	\qty[\qty(q-\ell)^{2}-m_{\ell_{k}}^{2}]\qty[\qty(p-\ell)^{2}-m_{\ell_{k}}^{2}]
	}
	\Delta^{\mu\nu}_{W}(\ell)
	\epsilon^{*}_{\alpha}(k)
	\\
	i\cA^{(c)}_{2}
	 & =
	-ieA^{*}B m^{2}_{\ell_{k}}
	\int\frac{\dd[4]{\ell}}{(2\pi)^{4}}
	\frac{
	x_{\nu}^{\dagger}(q)
	\bar{\sigma}_{\mu}\sigma_{\alpha}\bar{\sigma}_{\nu}
	x_{\rhn}(p)
	}{
	\qty[\qty(q-\ell)^{2}-m_{\ell_{k}}^{2}]\qty[\qty(p-\ell)^{2}-m_{\ell_{k}}^{2}]
	}
	\Delta^{\mu\nu}_{W}(\ell)
	\epsilon^{*}_{\alpha}(k)
	\\
	i\cA^{(d)}_{2}
	 & =
	ieAB^{*}m^{2}_{\ell_{k}}
	\int\frac{\dd[4]{\ell}}{(2\pi)^{4}}
	\frac{
	y_{\nu}(q)
	\sigma_{\mu}
	\bar{\sigma}_{\alpha}
	\sigma_{\nu}
	y_{\rhn}^{\dagger}(p)
	}{
	\qty[\qty(q-\ell)^{2}-m_{\ell_{k}}^{2}]\qty[\qty(p-\ell)^{2}-m_{\ell_{k}}^{2}]
	}
	\Delta^{\mu\nu}_{W}(\ell)
	\epsilon^{*}_{\alpha}(k)
\end{align}

% ============================================================================
% ---- L-Emission Diagrams with G --------------------------------------------
% ============================================================================

The amplitudes for the diagrams with Goldstones in \FigRef{fig:n_to_nu_gamma_ell} are given by
\begin{align}
	i\cA^{(e)}_{2}
	 & =
	-ie\tilde{A}\tilde{B}^{*}
	\int\frac{\dd[4]{\ell}}{(2\pi)^{4}}
	\frac{
	x_{\nu}^{\dagger}(q)
	\qty[\qty(q-\ell)\cdot\bar{\sigma}]\sigma_{\alpha}\qty[\qty(p-\ell)\cdot\bar{\sigma}]
	x_{\rhn}(p)
	}{
	\qty[\qty(q-\ell)^{2}-m_{\ell_{k}}^{2}]\qty[\qty(p-\ell)^{2}-m_{\ell_{k}}^{2}]
	}
	\Delta^{G}(\ell)
	\epsilon^{*}_{\alpha}(k)
	\\
	%--------------------------
	i\cA^{(f)}_{2}
	 & =
	-ie\tilde{A}^{*}\tilde{B}
	\int\frac{\dd[4]{\ell}}{(2\pi)^{4}}
	\frac{
	y_{\nu}(q)
	\qty[\qty(q-\ell)\cdot\sigma]\bar{\sigma}_{\alpha}\qty[\qty(p-\ell)\cdot\sigma]
	y_{\rhn}^{\dagger}(p)
	}{
	\qty[\qty(q-\ell)^{2}-m_{\ell_{k}}^{2}]\qty[\qty(p-\ell)^{2}-m_{\ell_{k}}^{2}]
	}
	\Delta^{G}(\ell)
	\epsilon^{*}_{\alpha}(k)
	\\
	i\cA^{(g)}_{2}
	 & =
	ie\tilde{A}\tilde{B}^{*}m^{2}_{\ell_{k}}
	\int\frac{\dd[4]{\ell}}{(2\pi)^{4}}
	\frac{
	x_{\nu}^{\dagger}(q)\bar{\sigma}_{\alpha}x_{\rhn}(p)
	}{
	\qty[\qty(q-\ell)^{2}-m_{\ell_{k}}^{2}]\qty[\qty(p-\ell)^{2}-m_{\ell_{k}}^{2}]
	}
	\Delta^{G}(\ell)
	\epsilon^{*}_{\alpha}(k)
	\\
	i\cA^{(h)}_{2}
	 & =
	-ie\tilde{A}^{*}\tilde{B}m^{2}_{\ell_{k}}
	\int\frac{\dd[4]{\ell}}{(2\pi)^{4}}
	\frac{
	y_{\nu}(q)\sigma_{\alpha}y_{\rhn}^{\dagger}(p)
	}{
	\qty[\qty(q-\ell)^{2}-m_{\ell_{k}}^{2}]\qty[\qty(p-\ell)^{2}-m_{\ell_{k}}^{2}]
	}
	\Delta^{G}(\ell)
	\epsilon^{*}_{\alpha}(k)
\end{align}
