# Supplementary material for: Sterile Neutrinos from Dark Matter: A $\nu$ Nightmare?
Source: arXiv:2211.05996 source file (2022-11-11)
Supplement: Supplementary file 13 [file ew_n_to_nu_gamma_fig1.tex]

\begin{figure}[ht!]
    \centering
    \begin{subfigure}[b]{0.45\linewidth}
        \begin{tikzpicture}
            \begin{feynman}
                \vertex (i1)  {\(\rhn_{i}\)};
                \vertex[right=1cm of i1] (v1) ;
                \vertex[right=1cm of v1] (g1) ;
                \vertex[right=1cm of g1] (v2) ;
                \vertex[above=1cm of g1] (v3) ;
                \vertex[right=1cm of v2] (o1) {\(\nu_{j}\)};
                \vertex[above=1cm of v3] (g2) ;
                \vertex[right=1cm of g2] (o2) {\(\gamma\)};
                \diagram*{
                (i1) -- [fermion] (v1) -- [fermion,edge label=\(\ell_{k}\)](v2) -- [fermion](o1);
                (v1) -- [charged boson,quarter left,looseness=1.0,edge label=\(W^{+}\)] (v3) -- [charged boson,quarter left,looseness=1.0] (v2);
                (v3) -- [boson] (o2);
                };
            \end{feynman}
        \end{tikzpicture}
        \caption{}
    \end{subfigure}
    \begin{subfigure}[b]{0.45\linewidth}
        \begin{tikzpicture}
            \begin{feynman}
                \vertex (i1)  {\(\rhn_{i}\)};
                \vertex[right=1cm of i1] (v1) ;
                \vertex[right=1cm of v1] (g1) ;
                \vertex[right=1cm of g1] (v2) ;
                \vertex[above=1cm of g1] (v3) ;
                \vertex[right=1cm of v2] (o1) {\(\nu_{j}\)};
                \vertex[above=1cm of v3] (g2) ;
                \vertex[right=1cm of g2] (o2) {\(\gamma\)};
                \diagram*{
                (o1) -- [fermion] (v2) -- [fermion](v1) -- [fermion](i1);
                (v1) -- [anti charged boson,quarter left,looseness=1.0] (v3) -- [anti charged boson,quarter left,looseness=1.0] (v2);
                (v3) -- [boson] (o2);
                };
            \end{feynman}
        \end{tikzpicture}
        \caption{}
    \end{subfigure}
    \begin{subfigure}[b]{0.45\linewidth}
        \begin{tikzpicture}
            \begin{feynman}
                \vertex (i1)  {\(\rhn_{i}\)};
                \vertex[right=1cm of i1] (v1) ;
                \vertex[right=1cm of v1] (g1) ;
                \vertex[right=1cm of g1] (v2) ;
                \vertex[above=1cm of g1] (v3) ;
                \vertex[right=1cm of v2] (o1) {\(\nu_{j}\)};
                \vertex[above=1cm of v3] (g2) ;
                \vertex[right=1cm of g2] (o2) {\(\gamma\)};
                \diagram*{
                (i1) -- [fermion] (v1) -- [anti fermion,edge label=\(\ell_{k}\)](v2) -- [fermion](o1);
                (v1) -- [anti charged scalar,quarter left,looseness=1.0,edge label=\(G^{+}\)] (v3) -- [anti charged scalar,quarter left,looseness=1.0] (v2);
                (v3) -- [boson] (o2);
                };
            \end{feynman}
        \end{tikzpicture}
        \caption{}
    \end{subfigure}
    \begin{subfigure}[b]{0.45\linewidth}
        \begin{tikzpicture}
            \begin{feynman}
                \vertex (i1)  {\(\rhn_{i}\)};
                \vertex[right=1cm of i1] (v1) ;
                \vertex[right=1cm of v1] (g1) ;
                \vertex[right=1cm of g1] (v2) ;
                \vertex[above=1cm of g1] (v3) ;
                \vertex[right=1cm of v2] (o1) {\(\nu_{j}\)};
                \vertex[above=1cm of v3] (g2) ;
                \vertex[right=1cm of g2] (o2) {\(\gamma\)};
                \diagram*{
                (o1) -- [fermion] (v2) -- [anti fermion](v1) -- [fermion](i1);
                (v1) -- [charged scalar,quarter left,looseness=1.0] (v3) -- [charged scalar,quarter left,looseness=1.0] (v2);
                (v3) -- [boson] (o2);
                };
            \end{feynman}
        \end{tikzpicture}
        \caption{}
    \end{subfigure}
    \caption{Diagrams contributing to \(\rhn_{i}\to\nu_{j}\gamma\) with photon
        emission from \(W\)-boson.}
    \label{fig:n_to_nu_gamma_w}
\end{figure}
