# Supplementary material for: Sterile Neutrinos from Dark Matter: A $\nu$ Nightmare?
Source: arXiv:2211.05996 source file (2022-11-11)
Supplement: Supplementary file 14 [file ew_n_to_nu_gamma_fig2.tex]

\begin{figure}[ht!]
    \centering
    \begin{subfigure}[b]{0.45\linewidth}
        \begin{tikzpicture}
            \begin{feynman}
                \vertex (i1)  {\(\rhn_{i}\)};
                \vertex[right=1cm of i1] (v1) ;
                \vertex[right=1cm of v1] (v2) ;
                \vertex[right=1cm of v2] (v3) ;
                \vertex[right=1cm of v3] (o1) {\(\nu_{j}\)};
                \vertex[below=1cm of v2] (g1) ;
                \vertex[right=1cm of g1] (o2) {\(\gamma\)};
                \diagram*{
                (i1) -- [fermion] (v1) -- [fermion,edge label'=\(\ell_{k}\)](v2) -- [fermion](v3) -- [fermion](o1);
                (v1) -- [charged boson,half left,looseness=1.5,edge label=\(W^{+}\)] (v3) ;
                (v2) -- [boson] (o2);
                };
            \end{feynman}
        \end{tikzpicture}
        \caption{}
    \end{subfigure}
    \begin{subfigure}[b]{0.45\linewidth}
        \begin{tikzpicture}
            \begin{feynman}
                \vertex (i1)  {\(\rhn_{i}\)};
                \vertex[right=1cm of i1] (v1) ;
                \vertex[right=1cm of v1] (v2) ;
                \vertex[right=1cm of v2] (v3) ;
                \vertex[right=1cm of v3] (o1) {\(\nu_{j}\)};
                \vertex[below=1cm of v2] (g1) ;
                \vertex[right=1cm of g1] (o2) {\(\gamma\)};
                \diagram*{
                (i1) -- [anti fermion] (v1) -- [anti fermion](v2) -- [anti fermion](v3) -- [anti fermion](o1);
                (v1) -- [anti charged boson,half left,looseness=1.5] (v3) ;
                (v2) -- [boson] (o2);
                };
            \end{feynman}
        \end{tikzpicture}
        \caption{}
    \end{subfigure}
    \begin{subfigure}[b]{0.45\linewidth}
        \begin{tikzpicture}
            \begin{feynman}
                \vertex (i1)  {\(\rhn_{i}\)};
                \vertex[right=1cm of i1] (v1) ;
                \vertex[right=1cm of v1] (v2) ;
                \vertex[right=1cm of v2] (v3) ;
                \vertex[right=1cm of v3] (o1) {\(\nu_{j}\)};
                \vertex[below=1cm of v2] (g3) ;
                \vertex[right=1cm of g3] (o2) {\(\gamma\)};
                \diagram*{
                (i1) -- [fermion] (v1) -- [majorana](v2) -- [anti majorana] (v3) -- [fermion](o1);
                (v1) -- [charged boson,half left,looseness=1.5] (v3) ;
                (v2) -- [boson] (o2);
                };
            \end{feynman}
        \end{tikzpicture}
        \caption{}
    \end{subfigure}
    \begin{subfigure}[b]{0.45\linewidth}
        \begin{tikzpicture}
            \begin{feynman}
                \vertex (i1)  {\(\rhn_{i}\)};
                \vertex[right=1cm of i1] (v1) ;
                \vertex[right=1cm of v1] (v2) ;
                \vertex[right=1cm of v2] (v3) ;
                \vertex[right=1cm of v3] (o1) {\(\nu_{j}\)};
                \vertex[below=1cm of v2] (g3) ;
                \vertex[right=1cm of g3] (o2) {\(\gamma\)};
                \diagram*{
                (i1) -- [anti fermion] (v1) -- [anti majorana](v2) -- [majorana] (v3) -- [anti fermion](o1);
                (v1) -- [anti charged boson,half left,looseness=1.5] (v3) ;
                (v2) -- [boson] (o2);
                };
            \end{feynman}
        \end{tikzpicture}
        \caption{}
    \end{subfigure}
    \begin{subfigure}[b]{0.45\linewidth}
        \begin{tikzpicture}
            \begin{feynman}
                \vertex (i1)  {\(\rhn_{i}\)};
                \vertex[right=1cm of i1] (v1) ;
                \vertex[right=1cm of v1] (v2) ;
                \vertex[right=1cm of v2] (v3) ;
                \vertex[right=1cm of v3] (o1) {\(\nu_{j}\)};
                \vertex[below=1cm of v2] (g1) ;
                \vertex[right=1cm of g1] (o2) {\(\gamma\)};
                \diagram*{
                (i1) -- [fermion] (v1) -- [anti fermion,edge label'=\(\ell_{k}\)](v2) -- [anti fermion](v3) -- [fermion](o1);
                (v1) -- [anti charged scalar,half left,looseness=1.5,edge label=\(G^{+}\)] (v3) ;
                (v2) -- [boson] (o2);
                };
            \end{feynman}
        \end{tikzpicture}
        \caption{}
    \end{subfigure}
    \begin{subfigure}[b]{0.45\linewidth}
        \begin{tikzpicture}
            \begin{feynman}
                \vertex (i1)  {\(\rhn_{i}\)};
                \vertex[right=1cm of i1] (v1) ;
                \vertex[right=1cm of v1] (v2) ;
                \vertex[right=1cm of v2] (v3) ;
                \vertex[right=1cm of v3] (o1) {\(\nu_{j}\)};
                \vertex[below=1cm of v2] (g1) ;
                \vertex[right=1cm of g1] (o2) {\(\gamma\)};
                \diagram*{
                (i1) -- [anti fermion] (v1) -- [fermion](v2) -- [fermion](v3) -- [anti fermion](o1);
                (v1) -- [charged scalar,half left,looseness=1.5] (v3) ;
                (v2) -- [boson] (o2);
                };
            \end{feynman}
        \end{tikzpicture}
        \caption{}
    \end{subfigure}
    \begin{subfigure}[b]{0.45\linewidth}
        \begin{tikzpicture}
            \begin{feynman}
                \vertex (i1)  {\(\rhn_{i}\)};
                \vertex[right=1cm of i1] (v1) ;
                \vertex[right=1cm of v1] (v2) ;
                \vertex[right=1cm of v2] (v3) ;
                \vertex[right=1cm of v3] (o1) {\(\nu_{j}\)};
                \vertex[below=1cm of v2] (g3) ;
                \vertex[right=1cm of g3] (o2) {\(\gamma\)};
                \diagram*{
                (i1) -- [fermion] (v1) -- [anti majorana](v2) -- [majorana] (v3) -- [fermion](o1);
                (v1) -- [anti charged scalar,half left,looseness=1.5] (v3) ;
                (v2) -- [boson] (o2);
                };
            \end{feynman}
        \end{tikzpicture}
        \caption{}
    \end{subfigure}
    \begin{subfigure}[b]{0.45\linewidth}
        \begin{tikzpicture}
            \begin{feynman}
                \vertex (i1)  {\(\rhn_{i}\)};
                \vertex[right=1cm of i1] (v1) ;
                \vertex[right=1cm of v1] (v2) ;
                \vertex[right=1cm of v2] (v3) ;
                \vertex[right=1cm of v3] (o1) {\(\nu_{j}\)};
                \vertex[below=1cm of v2] (g3) ;
                \vertex[right=1cm of g3] (o2) {\(\gamma\)};
                \diagram*{
                (i1) -- [anti fermion] (v1) -- [majorana](v2) -- [anti majorana] (v3) -- [anti fermion](o1);
                (v1) -- [charged scalar,half left,looseness=1.5] (v3) ;
                (v2) -- [boson] (o2);
                };
            \end{feynman}
        \end{tikzpicture}
        \caption{}
    \end{subfigure}
    \caption{Diagrams contributing to \(\rhn_{i}\to\nu_{j}\gamma\) with photon
        emission from charged lepton. Note diagrams use two-component spinors
        with (c), (d), (g) and (f) representing charged lepton mass insertions.}
    \label{fig:n_to_nu_gamma_ell}
\end{figure}
