# Supplementary material for: Sterile Neutrinos from Dark Matter: A $\nu$ Nightmare?
Source: arXiv:2211.05996 source file (2022-11-11)
Supplement: Supplementary file 15 [file ew_n_to_nu_h.tex]

The amplitude for \(\rhn_{i}(P) \to H(p_{h}) + \nu_j(p_{\nu})\) is given by:
\begin{align}
	\cM & = 2i \qty[G_{ij}y(p_{\nu})x(P) + G^{*}_{ij}x^{\dagger}(p_{\nu})y^{\dagger}(P)]
\end{align}
where \(G_{ij} = \qty(\bm{\cK}_{L}^{\dagger}\bm{\cK}_{R})_{ij}\). Squaring an summing
over spins, we find:
\begin{align}
	\frac{1}{2}\sum_{\mathrm{spins}}\qty|\cM|^2
	 & =
	4\qty[\qty(m_{\rhn}^2+m_{\nu_{j}}^2 - m_{h}^2) \qty|G_{ij}|^2 + 2m_{\rhn_{i}}m_{\nu_{j}}\Re(G_{ij}^2)]
\end{align}
The partial width is therefore:
\begin{align}
	\Gamma(\rhn_{i}\to \nu_{j}h)
	 & =
	\frac{\lambda^{1/2}(m^{2}_{\rhn_{i}},m_{\nu_{j}}^2,m_{h}^{2})}{16\pi v^{2}m^{3}_{\rhn^{2}_{i}}}
	\bigg{[}
	\qty(m_{\rhn_{i}}^4+m_{\nu_{j}}^4 - m_{h}^2\qty(m_{\rhn_{i}}^2+m_{\nu_{j}}^2) + 6m_{\rhn_{i}}^2m_{\nu_{j}}^2) \qty|G_{ij}|^2 \\
	 & \quad\quad + 2m_{\nu_{j}}m_{\rhn_{i}}\qty(2m_{\rhn_{i}}^2 + 2m_{\nu_{j}}^2 - m_{h}^2)\Re(G_{ij}^2)
	\bigg{]}\notag                                                                                                               \\
	 & \quad\times \theta(m_{\rhn_{i}}-m_{\nu_{j}}-m_{h})\notag
\end{align}
