# Supplementary material for: Sterile Neutrinos from Dark Matter: A $\nu$ Nightmare?
Source: arXiv:2211.05996 source file (2022-11-11)
Supplement: Supplementary file 16 [file ew_n_to_nu_z.tex]

The amplitude for \(\rhn_{i}(P) \to Z(p_{Z}) + \nu_j(p_{\nu})\) is given by:
\begin{align}
    \cM & = -iG_{ij} \frac{e}{c_{W}s_{W}}\qty[x^{\dagger}(p_{\nu})\bar{\sigma}_{\mu}x(P)
        - y^{\dagger}(P)\bar{\sigma}_{\mu}y(p_{\nu})]\epsilon^{*}_{\mu}
\end{align}
where \(G_{ij} = \qty(\OmegaVVb^{\dagger}\OmegaVNb)_{ij}\). Squaring and summing
over spins, we find:
\begin{align}
    \frac{1}{2}\sum_{\mathrm{spins}}\qty|\cM|^2
     & =
    \frac{e^{2}\qty|G_{ij}|^2}{s^{2}_{W}M_{W}^{2}}
    \qty(\qty(m_{\rhn_{i}}+m_{\nu_{i}})^{2}-M_{Z}^{2})
    \qty(\qty(m_{\rhn_{i}}-m_{\nu_{i}})^{2}+2M_{Z}^{2})
\end{align}
The partial width is therefore:
% prefactor \lambda^{1/2}(m^{2}_{\rhn_{i}},m_{1}^2,m_{2}^{2}) / (16\pi m^{3}_{\rhn^{2}_{i}})
\begin{align}
    \Gamma(\rhn_{i}\to \nu_{j}Z)
     & =
    \frac{e^{2}\lambda^{1/2}(m^{2}_{\rhn_{i}},m_{\nu_{j}}^2,M_{Z}^{2})}{16\pi s^{2}_{W}M^{2}_{W}m^{3}_{\rhn^{2}_{i}}}
    \qty|\qty(\OmegaVVb^{\dagger}\OmegaVNb)_{ij}|^2
    \qty(\qty(m_{\rhn_{i}}+m_{\nu_{i}})^{2}-M_{Z}^{2})\notag          \\
     & \quad\times\qty(\qty(m_{\rhn_{i}}-m_{\nu_{i}})^{2}+2M_{Z}^{2})
    \theta(m_{\rhn_{i}}-m_{\nu_{j}}-M_{Z})
\end{align}
