# Supplementary material for: Sterile Neutrinos from Dark Matter: A $\nu$ Nightmare?
Source: arXiv:2211.05996 source file (2022-11-11)
Supplement: Supplementary file 17 [file ew_three_body.tex]

\subsubsection{\texorpdfstring{\(\rhn_{i}\to\nu_{j}q\bar{q}\)}{RH-Neutrino to LH-Neutrino and Quarks}}
The amplitude for \(\rhn_{i}(P) \to \nu_{j}(p_{\nu}) + q(p_{q}) + \bar{q}(p_{\bar{q}})\), where
\(q \in \qty{u,c,t,d,s,b}\) is a SM quark, contains a Z and a Higgs exchanged diagram. The diagrams are given by:
\begin{align}
    i\cM
     & =
    \qty[iG_{ij}y_{\nu}x_{\rhn} + iG^{*}_{ij}x^{\dagger}_{\nu}y^{\dagger}_{\rhn}]
    \qty(i\Delta_{h})
    \qty(-i\frac{m_{q}}{v})
    \qty[x^{\dagger}_{q}x^{\dagger}_{\bar{q}} + y_{u}y_{\bar{q}}] \\
     & \quad +
    \qty(i\tilde{G}_{ij})
    \qty[x^{\dagger}_{\nu}\bar{\sigma}^{\mu}x_{\rhn} - y^{\dagger}_{\rhn}\bar{\sigma}^{\mu}y_{\nu}]
    \qty(i\Delta^{\mu\nu}_{Z})
    \qty[ig^{q}_{L}x^{\dagger}_{q}\bar{\sigma}^{\mu}y_{\bar{q}} -ig^{q}_{R}x^{\dagger}_{\bar{q}}\bar{\sigma}^{\mu}y_{q}]
\end{align}
where \(G_{ij} = \qty(\OmegaNNb^{T}\hat{\bm{m}}\OmegaNVb)_{ij}\),
\(\tilde{G}_{ij} = (e/c_{W}s_{W})\qty(\OmegaVVb^{\dagger}\OmegaVN)_{ij}\) and the left and right handed
quark couplings to the Z are:
\begin{align}
    g^{q}_{L} & = \frac{e}{c_{W}s_{W}}\qty(T^{3}_{q} - s^{2}_{W}Q_{q}), &
    g^{q}_{R} & = \frac{e s_{W}}{c_{W}}Q_{q}
\end{align}
with \(T^{3}_{u} = 1/2, Q_{u}=2/3\) for up-type quarks and
\(T^{3}_{d} = -1/2, Q_{d}=-1/3\) for down-type quarks.
\(\Delta_{h}\) and \(\Delta^{\mu\nu}_{Z}\) are propagators for the Higgs and
Z-boson (in the unitary gauge) given by:
\begin{align}
    \Delta_{h}(p)
                                                   & =
    \frac{1}{p^2 - M^{2}_{h} + i M_{h}\Gamma_{h}}, &
    \Delta^{\mu\nu}_{Z}(p)
                                                   & =
    \frac{1}{p^2 - M^{2}_{Z} + i M_{Z}\Gamma_{Z}}
    \qty(-g^{\mu\nu} + \frac{p^{\mu}p^{\nu}}{M^{2}_{Z}})
\end{align}
Squaring and summing over spins, we find:
\begin{align}
    \frac{1}{2}\sum_{\mathrm{spins}}\qty|\cM|^2
     & =
    \frac{1}{2}\qty(
    N Q \qty|\Delta_{h}|^{2}
    + \qty[N_{\mu}Q_{\nu}\Delta^{\mu\nu}_{Z}\qty(\Delta_{H})^{*} + \mathrm{c.c}]
    + N_{\mu\alpha} Q_{\nu\beta}\Delta_{Z}^{\mu\nu}\qty(\Delta_{Z}^{\alpha\beta})^{*}
    )
\end{align}
where
\begin{align}
    N
     & =
    2\qty(
    \Re(G^{2}_{ij})m_{\nu_{j}}m_{\rhn_{i}}+4\qty|G_{ij}|^{2}\qty(P\cdot p_{\nu})
    )
    \\
    Q
     & = -\frac{4m^{2}_{u_{k}}}{v^{2}}\qty(m^{2}_{u_{k}} - p_{u}p_{\bar{u}})
    \\
    N^{\mu}
     & =
    \frac{2e}{c_{W}s_{W}}\qty(
    \mathrm{Im}\qty(G_{ij}\qty(\tilde{G}_{ij})^{*})m_{\nu_{j}}P^{\mu}
    - m_{\rhn_{i}}\Im(G_{ij}\tilde{G}_{ij})p^{\mu}_{\nu}
    )
    \\
    Q^{\mu}
     & =
    \frac{2m_{u_{k}}^{2}}{v}\qty(g_{L,q}-g_{R,q})(p^{\mu}_{u}-p^{\mu}_{\bar{u}})
    \\
    N^{\mu\alpha}
     & =
    -2\qty(
    2\Re(\tilde{G}_{ij})m_{\nu_{j}}m_{\rhn_{i}}g^{\mu\alpha}
    -2\qty|\tilde{G}_{ij}|^{2}\qty(
    P^{\alpha}p^{\mu}_{\nu} +
    P^{\mu}p^{\alpha}_{\nu}-\qty(P\cdot p_{\nu})g^{\mu\alpha}
    )
    )                                                                        \\
    Q^{\nu\beta}
     & =
    2\qty(g^{2}_{L,q} + g^{2}_{R,q})
    \qty(
    p^{\nu}_{u}p^{\beta}_{\bar{u}} +
    p^{\beta}_{u}p^{\nu}_{\bar{u}}
    )
    -2\qty(\qty(g^{2}_{L,q} + g^{2}_{R,q})\qty(p_{u}\cdot p_{\bar{u}})
    -2g_{L,q}g_{R,q}m^{2}_{u_{k}}
    )
\end{align}
